# Supplementary material for: Structured Pruning for Deep Convolutional Neural Networks: A survey
Source: arXiv:2303.00566 source file (2023-11-30)
Supplement: Supplementary file 1 [file supp.pdf]

# Supplementary for Structured Pruning for Deep Convolutional Neural Networks: A survey

Yang He, Lingao Xiao

## 1 Related Works

**Unstructured Pruning (Weight Pruning):** The idea of pruning is first introduced by LeCun *et al.* [1] who propose *saliency* to measure the importance of each weight. The *saliency* is computed by the diagonal elements of the Hessian matrix. Han *et al.* [2] propose to iteratively prune weights with $\ell_1$ regularization and retrain. Guo *et al.* [3] propose *connection splicing* which restores the wrongly pruned weights. In addition, Guo *et al.* incorporate the *connection splicing* into the training process to dynamically learn the weights [3]. Han *et al.* [4] adopt a 3-stage pipeline to prune weights and achieve a 49× compression ratio with merely accuracy loss on VGG-16 [5], bringing back the research focus on network pruning.

**Quantization:** Quantization in model compression describes the process of approximating full precision weights (*32-bit floating point*) with lower precision weights (e.g., *8-bit integer*) to reduce computation and storage cost. The low-bit quantization includes binarization [6], [7] and ternarization [8], [9]. These methods can be roughly divided into two categories. First, heuristic quantization methods quantize weights by using mapping functions [7], [8]. Second, non-heuristic methods formulate quantization as an optimization problem [6], [9]. In addition, the quantization process also includes clustering and parameter sharing [10], and quantization can be combined with pruning [4], [11], [12].

**Decomposition:** Decomposition is referring to matrix decomposition and tensor decomposition, where a matrix is just a 2-D tensor. Specifically, a tensor is decomposed or factorized into products of several low-rank tensors that approximate the original tensor. To decompose 2-D tensors (matrices), *full-rank decomposition* [13], *singular value decomposition (SVD)* [14], and *QR* [15] are arguably the most popular low-rank matrix decomposition techniques. To deal with 4-D tensors, methods or concepts such as *Tucker* [16], *classical prolongation (CP)* [17], and *tensor networks* [18] are applied. Furthermore, decomposition is orthogonal to pruning, and these two techniques are applied together [19], [20], [21].

**Knowledge Distillation:** The idea of transferring knowledge from a usually large network to a small network is first introduced by Bucilua *et al.* [22], and the idea is later well-known as Knowledge Distillation [23]. The distillation process includes *(1) offline distillation* [23] which takes a pre-trained teacher model. Distillation can also be *(2) online distillation* [24] which simultaneously updates the teacher model and the student model in an end-to-end manner. Furthermore, *(3) self-distillation* [25] requires only one model and distills the knowledge from deeper sections to shallow sections. In addition, knowledge distillation can work with pruning to achieve few-shot compression which requires few data [26], [27], [28].

**Neural Architecture Search:** The objective of neural architecture search [29] is to minimize human intervention in the search for neural network designs. In this regard, three factors play a significant role. (1) The search space defines potential candidates. Selecting candidates with prior knowledge reduces the frequently vast search space, but human bias may hinder performance. (2) Search strategies are the search space exploration algorithms. Simple taxonomy involves Bayesian optimization [30], evolutionary methods [31], gradient-based methods [32], and reinforcement learning [33]. (3) The evaluation strategy is used to assess the predictive ability of the model on unseen data. To address the prohibitive computational cost of the model's evaluation, efficient methods are developed.

## 2 Experiments

We summarize 800+ experiment results from 100+ papers into **21 tables** over the three most popular datasets: CIFAR-10, CIFAR-100, and ImageNet-1K. The detailed numbers of covered methods, models and results are summarized in Tab. 1. The 21 tables are easily accessible via the links in Tab. 2.

In each table, we specify their corresponding sections and the years they were published in each table. Note that various methods adopt distinct settings for baselines and fine-tuning. To offer a comprehensive contrast, we present nine metrics for these methods:

1) Baseline Accuracy
2) Accuracy After Pruning
3) Accuracy Drop (%)
4) Baseline FLOPs
5) FLOPs After Pruning
6) FLOPs Drop (%)
7) Baseline Parameters
8) Parameters After Pruning
9) Parameters Drop (%)

| Section | 2.1.1 | 2.1.2 | 2.2.1 | 2.2.2 | 2.2.3 | 2.3.1 | 2.3.2 | 2.3.3 | 2.4.1 | 2.4.2 | 2.4.3 | 2.5.1 | 2.5.2 | 2.6.1 | 2.6.2 | 2.6.3 | 2.7.1 | 2.7.2 | 2.7.3 | Total |
|---|---|---|---|---|---|---|---|---|---|---|---|---|---|---|---|---|---|---|---|---|
| #. methods | 1 | 5 | 4 | 3 | 4 | 6 | 9 | 3 | 6 | 4 | 4 | 7 | 6 | 6 | 11 | 4 | 6 | 6 | 7 | 102 |
| #. models | 4 | 11 | 9 | 9 | 13 | 9 | 12 | 7 | 12 | 8 | 10 | 13 | 10 | 13 | 13 | 11 | 9 | 13 | 10 | 27* |
| #. results | 7 | 30 | 53 | 30 | 36 | 44 | 72 | 26 | 62 | 18 | 19 | 71 | 39 | 51 | 99 | 45 | 33 | 38 | 35 | 808 |

TABLE 1: Summary of experiments in 21 tables. * denotes the unique models.

| | | |
|---|---|---|
| CIFAR-10 | VGG | VGG-16, VGG-19 |
| | ResNet (Small) | ResNet-20, ResNet-32, ResNet-44, ResNet-56, ResNet-110, ResNet-164 |
| | ResNet (Large) | ResNet-18, ResNet-34, ResNet-50, ResNet-101 |
| | MobileNet | MobileNet-V1, MobileNet-V2 |
| | Other | DenseNet-40, GoogLeNet, PreResNet-29, PreResNet-101, ResNeXt-20, ResNeXt-164, NAS |
| CIFAR-100 | VGG | VGG-16, VGG-19 |
| | ResNet (Small) | ResNet-20, ResNet-32, ResNet-44, ResNet-56, ResNet-110, ResNet-164 |
| | ResNet (Large) | ResNet-18, ResNet-34, ResNet-50, ResNet-101 |
| | MobileNet | MobileNet-V1, MobileNet-V2 |
| | Other | DenseNet-40, PreResNet-29, PreResNet-101, ResNeXt-20, ResNeXt-164 |
| ImageNet-1K | AlexNet | AlexNet |
| | VGG | VGG-11, VGG-16 |
| | ResNet | ResNet-18, ResNet-34, ResNet-50, ResNet-101, ResNet-152 |
| | MobileNet | MobileNet-V1, MobileNet-V2, MobileNet-V3-Small |
| | Other | ProxylessNet-Mobile, GoogLeNet, ResNeXt-50, NAS |

TABLE 2: Indexing of the 21 tables.

For papers that only report the FLOPs drop ratio without a baseline, we determine the pruned model's absolute FLOPs using our calculation of the FLOPs baseline. We apply a similar approach to the parameter count. Tables are sorted according to the FLOPs of pruned models.

## 3 Our Website

To better visualize and analyze the experiment results, we have developed a dedicated website that offers a more interactive and dynamic platform for comparing structured pruning methods. The website is available at: https://huggingface.co/spaces/he-yang/Structured-Pruning-Survey.

We provide an illustrative example in Fig. 1 to show how the query works. If a user wants to find methods that satisfy the following:

1) Select Dataset: ImageNet-1K
2) Select Model: ResNet-50
3) Select Pruning Method: Regularization-based Pruning in section 2.3
4) Target 1: Accuracy after pruning $> 75\%$
5) Target 2: Pruned FLOPs $> 40\%$
6) Target 3: Model size after pruning $< 30$M

By simply entering the requirements into the corresponding query box, we can narrow down the results to five data points from three methods, including GBN, SCOP, and OTO. If we click the method name, such as SCOP, the corresponding paper title, link, code, venues and BibTeX for this method will be generated.

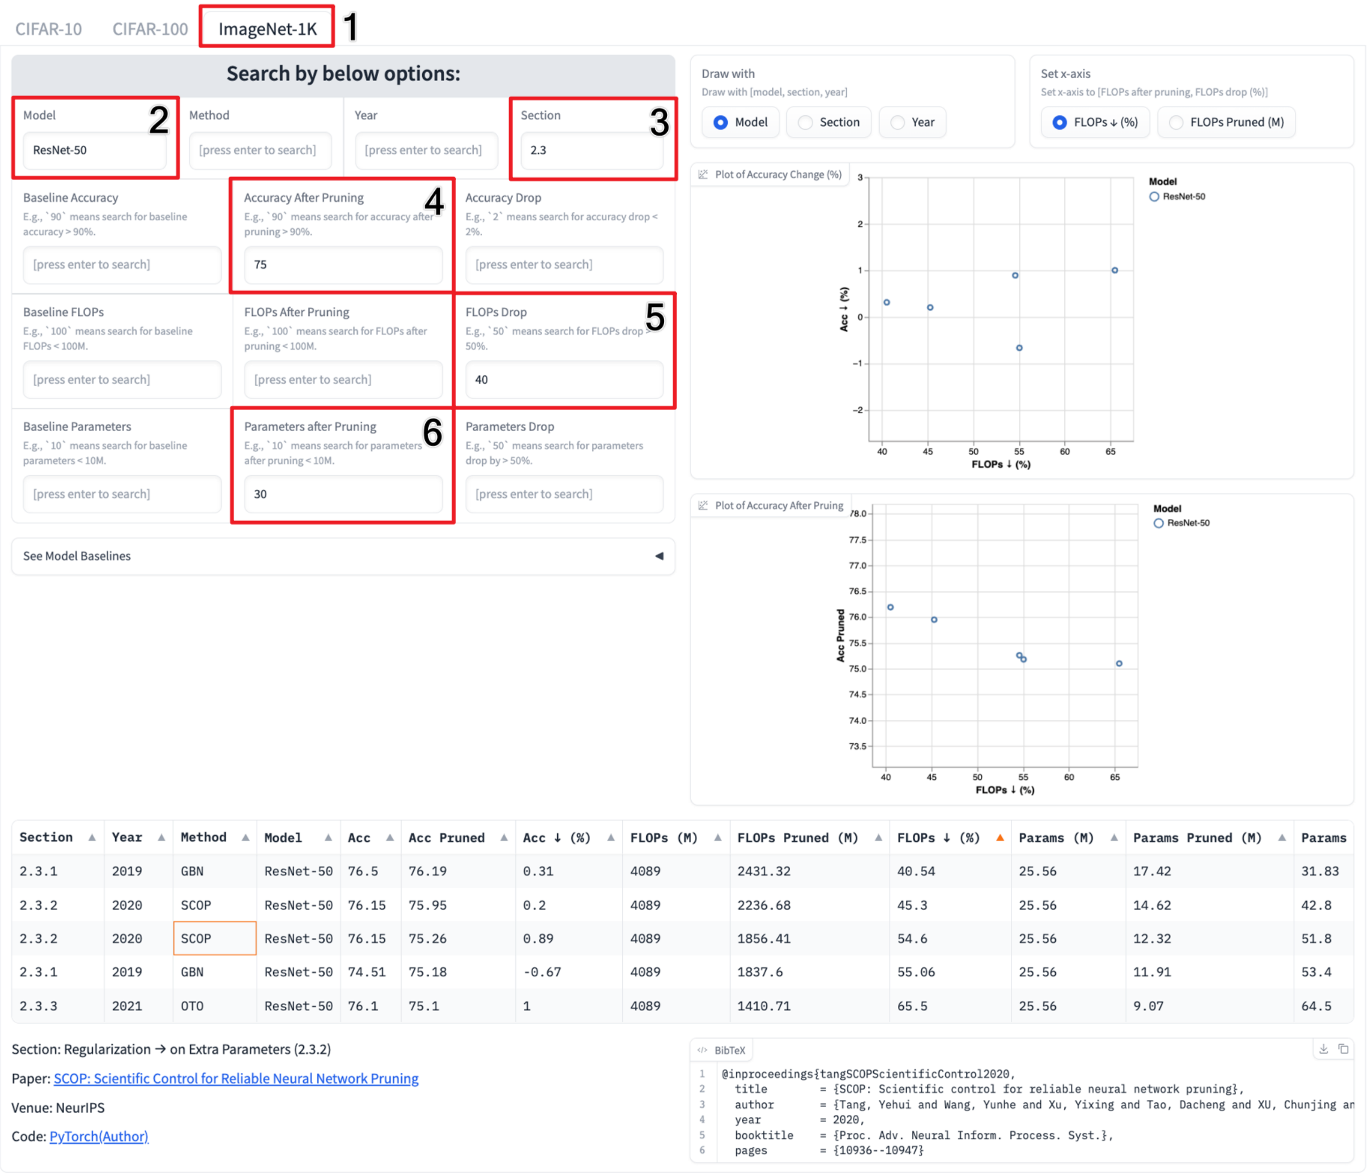


Fig. 1: An illustrative example sourced from our website: https://huggingface.co/spaces/he-yang/Structured-Pruning-Survey.

| Section | Year | Method | Baseline Top-1 Acc.(%) | Pruned Top-1 Acc.(%) | Top-1 Acc. ↓(%) | Baseline FLOPs (M) | Pruned FLOPs (M) | FLOPs ↓(%) | Baseline Params (M) | Pruned Params (M) | Params ↓(%) |
|---|---|---|---|---|---|---|---|---|---|---|---|
| VGG-16 | | | | | | | | | | | |
| 2.6.1 | 2020 | AutoCompress [34] | 93.70 | 93.21 | -0.49 | 314.59 | 35.75 | 88.64 | 14.73 | - | - |
| 2.6.1 | 2022 | DECORE [35] | 93.96 | 91.68 | -2.28 | 314.59 | 36.95 | 88.25 | 14.73 | 0.26 | 98.26 |
| 2.4.3 | 2022 | StructADMM [36] | - | 93.10 | - | 314.59 | 37.90 | 87.95 | 14.73 | - | - |
| 2.2.3 | 2020 | PFP [37] | 92.89 | 92.39 | -0.50 | 314.59 | 47.09 | 85.03 | 14.73 | 0.84 | 94.32 |
| 2.3.3 | 2021 | OTO [38] | 91.60 | 91.00 | -0.60 | 314.59 | 51.28 | 83.70 | 14.73 | 0.37 | 97.50 |
| 2.6.1 | 2022 | DECORE [35] | 93.96 | 92.44 | -1.52 | 314.59 | 51.34 | 83.68 | 14.73 | 0.50 | 96.60 |
| 2.3.2 | 2021 | ABP [39] | 93.96 | 92.65 | -1.31 | 314.59 | 52.81 | 83.21 | 14.73 | 1.50 | 89.79 |
| 2.7.2 | 2021 | EDP [40] | 93.60 | 93.52 | -0.08 | 314.59 | 62.57 | 80.11 | 14.73 | 0.65 | 95.59 |
| 2.6.1 | 2022 | RL-MCTS [41] | 93.51 | 93.72 | 0.21 | 314.59 | 63.23 | 79.90 | 14.73 | - | - |
| 2.2.1 | 2021 | CHIP [42] | 93.96 | 93.18 | -0.78 | 314.59 | 67.32 | 78.60 | 14.73 | 1.87 | 87.30 |
| 2.4.2 | 2018 | VIBNet [43] | - | 91.50 | - | 314.59 | 70.99 | 77.43 | 14.73 | 0.78 | 94.70 |
| 2.2.3 | 2022 | DLRFC [44] | 93.25 | 93.64 | -0.39 | 314.59 | 72.51 | 76.95 | 14.73 | 0.83 | 94.38 |
| 2.2.1 | 2020 | HRank [45] | 93.96 | 91.23 | -2.73 | 314.59 | 73.90 | 76.51 | 14.73 | 1.75 | 88.12 |
| 2.3.2 | 2022 | WhiteBox [46] | 93.02 | 93.47 | 0.45 | 314.59 | 74.24 | 76.40 | 14.73 | - | - |
| 2.1.2 | 2022 | EPruner [47] | 93.02 | 93.08 | 0.06 | 314.59 | 74.42 | 76.34 | 14.73 | 1.65 | 88.80 |
| 2.2.2 | 2019 | AOFP [48] | 93.38 | 93.28 | -0.10 | 314.59 | 77.39 | 75.40 | 14.73 | - | - |
| 2.1.2 | 2022 | CLR-RNF [49] | 93.02 | 93.32 | 0.30 | 314.59 | 81.48 | 74.10 | 14.73 | 0.74 | 95.00 |
| 2.6.3 | 2020 | ABCPruner [50] | 93.02 | 93.08 | 0.06 | 314.59 | 82.81 | 73.68 | 14.73 | 1.67 | 88.66 |
| 2.1.2 | 2019 | COP [51] | 93.56 | 93.31 | -0.25 | 314.59 | 83.37 | 73.50 | 14.73 | 1.06 | 92.80 |
| 2.3.3 | 2021 | OTO [38] | 93.20 | 93.30 | 0.10 | 314.59 | 84.31 | 73.20 | 14.73 | 0.81 | 94.50 |
| 2.2.1 | 2022 | GCNP [52] | 93.10 | 93.08 | -0.02 | 314.59 | 84.72 | 73.07 | 14.73 | 1.02 | 93.06 |
| 2.5.2 | 2022 | FTWT [53] | 93.82 | 93.19 | -0.63 | 314.59 | 84.94 | 73.00 | 14.73 | - | - |
| 2.4.2 | 2018 | VIBNet [43] | - | 93.90 | - | 314.59 | 87.26 | 72.26 | 14.73 | 0.80 | 94.55 |
| 2.7.3 | 2022 | SOKS [54] | 93.53 | 94.01 | 0.48 | 314.59 | 87.46 | 72.20 | 14.73 | 3.19 | 78.33 |
| 2.4.2 | 2019 | RBP [55] | - | 91.00 | - | 314.59 | 89.88 | 71.43 | 14.73 | - | - |
| 2.7.3 | 2020 | SWP [56] | 93.25 | 93.65 | 0.40 | 314.59 | 90.73 | 71.16 | 14.73 | 1.08 | 92.66 |
| 2.3.2 | 2021 | GDP-Guo [57] | 93.89 | 93.99 | 0.10 | 314.59 | 96.11 | 69.45 | 14.73 | - | - |
| 2.2.1 | 2021 | CHIP [42] | 93.96 | 93.72 | -0.24 | 314.59 | 105.07 | 66.60 | 14.73 | 2.46 | 83.30 |
| 2.3.1 | 2020 | SCP [58] | 93.85 | 93.79 | 0.06 | 314.59 | 106.24 | 66.23 | 14.73 | 1.02 | 93.05 |
| 2.3.2 | 2021 | ABP [39] | 93.96 | 93.50 | -0.46 | 314.59 | 106.59 | 66.12 | 14.73 | 2.66 | 81.96 |
| 2.2.2 | 2019 | AOFP [48] | 93.38 | 93.47 | 0.09 | 314.59 | 108.55 | 65.50 | 14.73 | - | - |
| 2.2.1 | 2020 | HRank [45] | 93.96 | 92.34 | -1.62 | 314.59 | 108.91 | 65.38 | 14.73 | 2.60 | 82.38 |
| 2.5.2 | 2022 | FTWT [53] | 93.82 | 93.55 | -0.27 | 314.59 | 110.11 | 65.00 | 14.73 | - | - |
| 2.6.1 | 2022 | DECORE [35] | 93.96 | 93.56 | -0.40 | 314.59 | 110.81 | 64.78 | 14.73 | 1.63 | 88.92 |
| 2.6.3 | 2022 | CCEP [59] | 93.71 | 93.52 | -0.19 | 314.59 | 115.77 | 63.20 | 14.73 | - | - |
| 2.4.2 | 2018 | VIBNet [43] | - | 94.20 | - | 314.59 | 116.59 | 62.94 | 14.73 | 0.85 | 94.21 |
| 2.2.3 | 2022 | DLRFC [44] | 93.25 | 93.93 | -0.68 | 314.59 | 121.97 | 61.23 | 14.73 | 1.05 | 92.86 |
| 2.7.2 | 2021 | CC [60] | 93.70 | 94.09 | 0.39 | 314.59 | 123.62 | 60.70 | 14.73 | 4.02 | 72.69 |
| 2.7.3 | 2022 | SOKS [54] | 93.53 | 94.11 | 0.58 | 314.59 | 124.23 | 60.51 | 14.73 | 4.50 | 69.47 |
| 2.2.2 | 2019 | AOFP [48] | 93.38 | 93.84 | 0.46 | 314.59 | 124.63 | 60.38 | 14.73 | - | - |
| 2.2.1 | 2021 | CHIP [42] | 93.96 | 93.86 | -0.10 | 314.59 | 131.81 | 58.10 | 14.73 | 2.71 | 81.60 |
| 2.2.1 | 2022 | GCNP [52] | 93.10 | 93.27 | 0.17 | 314.59 | 134.36 | 57.29 | 14.73 | 2.14 | 85.50 |
| 2.6.2 | 2021 | EE [61] | 93.36 | 93.63 | 0.27 | 314.59 | 136.53 | 56.60 | 14.73 | - | - |
| 2.5.2 | 2022 | FTWT [53] | 93.82 | 93.73 | -0.09 | 314.59 | 138.42 | 56.00 | 14.73 | - | - |
| 2.3.1 | 2020 | PR [62] | 93.88 | 93.92 | -0.04 | 314.59 | 144.71 | 54.00 | 14.73 | - | - |
| 2.2.1 | 2020 | HRank [45] | 93.96 | 93.43 | -0.53 | 314.59 | 146.01 | 53.59 | 14.73 | 2.47 | 83.24 |
| 2.3.2 | 2021 | ABP [39] | 93.96 | 93.75 | -0.21 | 314.59 | 146.19 | 53.53 | 14.73 | 2.44 | 83.46 |
| 2.7.2 | 2021 | CC [60] | 93.70 | 94.15 | 0.45 | 314.59 | 154.78 | 50.80 | 14.73 | 5.02 | 65.90 |
| 2.6.1 | 2022 | RL-MCTS [41] | 93.51 | 93.90 | 0.39 | 314.59 | 171.45 | 45.50 | 14.73 | - | - |
| 2.3.2 | 2019 | GAL [63] | 93.96 | 90.78 | -3.18 | 314.59 | 172.36 | 45.21 | 14.73 | 2.63 | 82.18 |
| 2.3.2 | 2019 | GAL [63] | 93.96 | 93.42 | -0.54 | 314.59 | 172.36 | 45.21 | 14.73 | 2.63 | 82.18 |
| 2.7.1 | 2020 | EB [64] | - | 92.49 | - | 314.59 | 174.77 | 44.44 | 14.73 | 4.42 | 70.00 |
| 2.2.2 | 2019 | AOFP [48] | 93.38 | 94.03 | 0.65 | 314.59 | 186.94 | 40.58 | 14.73 | - | - |
| 2.3.2 | 2019 | GAL [63] | 93.96 | 93.77 | -0.19 | 314.59 | 190.01 | 39.60 | 14.73 | 3.30 | 77.57 |
| 2.3.2 | 2019 | GAL [63] | 93.96 | 92.03 | -1.93 | 314.59 | 190.01 | 39.60 | 14.73 | 3.30 | 77.57 |
| 2.4.2 | 2019 | VP [65] | 93.25 | 93.18 | -0.07 | 314.59 | 190.97 | 39.30 | 14.73 | 3.93 | 73.35 |
| 2.7.2 | 2020 | Hinge [66] | 94.02 | 93.59 | -0.43 | 314.59 | 191.68 | 39.07 | 14.73 | 2.94 | 80.05 |
| 2.7.3 | 2019 | SDN [67] | 93.50 | 93.47 | -0.03 | 314.59 | 192.21 | 38.90 | 14.73 | 1.78 | 87.90 |
| 2.2.1 | 2021 | LRMF [68] | 93.58 | 93.70 | 0.12 | 314.59 | 201.65 | 35.90 | 14.73 | - | - |
| 2.2.1 | 2021 | LRMF [68] | 93.58 | 93.20 | -0.38 | 314.59 | 201.65 | 35.90 | 14.73 | - | - |
| 2.6.1 | 2022 | DECORE [35] | 93.96 | 94.02 | 0.06 | 314.59 | 203.64 | 35.27 | 14.73 | 5.45 | 63.02 |
| 2.1.1 | 2017 | PFEC [69] | 93.25 | 93.40 | 0.15 | 314.59 | 207.05 | 34.19 | 14.73 | 5.30 | 64.00 |
| 2.2.2 | 2019 | AOFP [48] | 93.38 | 93.81 | 0.43 | 314.59 | 216.09 | 31.31 | 14.73 | - | - |
| 2.7.1 | 2020 | EB [64] | - | 93.90 | - | 314.59 | 224.71 | 28.57 | 14.73 | 7.37 | 50.00 |
| 2.7.1 | 2020 | EB [64] | - | 93.91 | - | 314.59 | 262.16 | 16.67 | 14.73 | 10.31 | 30.00 |
| 2.7.1 | 2022 | EarlyCroP [70] | 90.20 | 93.00 | 2.80 | 314.59 | - | - | 14.73 | 0.29 | 98.00 |
| 2.7.3 | 2022 | DPP [71] | 93.50 | 93.60 | 0.10 | 314.59 | - | - | 14.73 | 1.58 | 89.27 |

TABLE 3: VGG-16 on CIFAR-10.

| Section | Year | Method | Baseline Top-1 Acc.(%) | Pruned Top-1 Acc.(%) | Top-1 Acc. ↓(%) | Baseline FLOPs (M) | Pruned FLOPs (M) | FLOPs ↓(%) | Baseline Params (M) | Pruned Params (M) | Params ↓(%) |
|---|---|---|---|---|---|---|---|---|---|---|---|
| VGG-19 | | | | | | | | | | | |
| 2.6.1 | 2022 | DECORE [35] | 93.76 | 91.65 | -2.11 | 398.00 | 43.85 | 88.98 | 20.04 | 0.30 | 98.50 |
| 2.4.1 | 2019 | ED [72] | 94.17 | 92.29 | -1.88 | 398.00 | 53.69 | 86.51 | 20.04 | 0.57 | 97.15 |
| 2.5.1 | 2021 | SEP [73] | 93.66 | 93.40 | -0.26 | 398.00 | 59.80 | 84.97 | 20.04 | 4.01 | 79.99 |
| 2.4.1 | 2019 | ED [72] | 93.71 | 91.79 | -1.92 | 398.00 | 60.42 | 84.82 | 20.04 | 0.63 | 96.84 |
| 2.3.1 | 2020 | SCP [58] | 93.84 | 93.82 | 0.02 | 398.00 | 103.24 | 74.06 | 20.04 | 0.96 | 95.21 |
| 2.2.3 | 2018 | DCP [74] | 93.99 | 94.57 | 0.58 | 398.00 | 139.16 | 65.03 | 20.04 | 1.29 | 93.58 |
| 2.4.1 | 2022 | SOSP [75] | 94.18 | 93.73 | -0.45 | 398.00 | 168.19 | 57.74 | 20.04 | 2.55 | 87.29 |
| 2.5.1 | 2021 | DCP-CAC [76] | 92.47 | 93.19 | 0.72 | 398.00 | 195.00 | 51.01 | 20.04 | 5.51 | 72.53 |
| 2.3.1 | 2017 | NS [77] | 93.66 | 93.80 | 0.14 | 398.00 | 196.98 | 50.51 | 20.04 | 2.30 | 88.52 |
| 2.2.3 | 2018 | DCP [74] | 93.99 | 94.16 | 0.17 | 398.00 | 199.00 | 50.00 | 20.04 | 10.44 | 47.92 |
| 2.4.1 | 2022 | SOSP [75] | 94.18 | 93.99 | -0.19 | 398.00 | 215.08 | 45.96 | 20.04 | 2.86 | 85.75 |
| 2.4.1 | 2019 | ED [72] | 93.71 | 93.88 | 0.17 | 398.00 | 239.44 | 39.84 | 20.04 | 4.11 | 79.50 |
| 2.4.1 | 2019 | ED [72] | 94.17 | 93.98 | -0.19 | 398.00 | 250.22 | 37.13 | 20.04 | 4.37 | 78.18 |
| 2.7.1 | 2022 | ProsPr [78] | 93.60 | 93.61 | 0.01 | 398.00 | - | - | 20.04 | 4.01 | 80.00 |
| 2.7.1 | 2022 | ProsPr [78] | 93.60 | 93.64 | 0.04 | 398.00 | - | - | 20.04 | 2.00 | 90.00 |
| 2.7.1 | 2022 | ProsPr [78] | 93.60 | 93.32 | -0.28 | 398.00 | - | - | 20.04 | 1.00 | 95.00 |

TABLE 4: VGG-19 on CIFAR-10.

| Section | Year | Method | Baseline Top-1 Acc.(%) | Pruned Top-1 Acc.(%) | Top-1 Acc. ↓(%) | Baseline FLOPs (M) | Pruned FLOPs (M) | FLOPs ↓(%) | Baseline Params (M) | Pruned Params (M) | Params ↓(%) |
|---|---|---|---|---|---|---|---|---|---|---|---|
| ResNet-20 | | | | | | | | | | | |
| 2.6.2 | 2020 | DSA [79] | 92.17 | 90.24 | -1.93 | 40.81 | 13.26 | 67.50 | 0.27 | - | - |
| 2.7.3 | 2022 | SOKS [54] | 92.05 | 90.78 | -1.27 | 40.81 | 15.49 | 62.04 | 0.27 | 0.14 | 48.15 |
| 2.3.2 | 2020 | SCOP [80] | 92.22 | 90.75 | -1.47 | 40.81 | 18.08 | 55.70 | 0.27 | 0.12 | 56.30 |
| 2.7.2 | 2020 | Hinge [66] | 92.54 | 91.84 | -0.70 | 40.81 | 18.57 | 54.50 | 0.27 | 0.12 | 55.45 |
| 2.5.2 | 2021 | ManiDP [81] | 92.22 | 92.05 | -0.17 | 40.81 | 18.69 | 54.20 | 0.27 | - | - |
| 2.2.1 | 2021 | LRMF [68] | 92.20 | 90.47 | -1.73 | 40.81 | 18.77 | 54.00 | 0.27 | - | - |
| 2.1.2 | 2019 | FPGM [82] | 92.20 | 91.99 | -0.21 | 40.81 | 18.77 | 54.00 | 0.27 | - | - |
| 2.5.2 | 2021 | DDG [83] | 92.24 | 91.90 | -0.34 | 40.81 | 19.43 | 52.40 | 0.27 | - | - |
| 2.6.2 | 2022 | DAIS [84] | 93.25 | 92.89 | -0.36 | 40.81 | 19.96 | 51.10 | 0.27 | - | - |
| 2.6.1 | 2022 | GNN-RL [85] | 91.73 | 91.31 | -0.42 | 40.81 | 20.00 | 51.00 | 0.27 | - | - |
| 2.2.1 | 2022 | GCNP [52] | 92.25 | 91.58 | -0.67 | 40.81 | 20.18 | 50.54 | 0.27 | 0.17 | 38.51 |
| 2.6.2 | 2020 | DSA [79] | 92.17 | 91.38 | -0.79 | 40.81 | 20.28 | 50.30 | 0.27 | - | - |
| 2.6.1 | 2021 | AGMC [86] | 91.73 | 91.42 | -0.31 | 40.81 | 20.41 | 50.00 | 0.27 | - | - |
| 2.3.2 | 2021 | ABP [39] | 92.15 | 91.03 | -1.12 | 40.81 | 21.34 | 47.70 | 0.27 | 0.15 | 45.10 |
| 2.1.2 | 2021 | SRR [87] | 92.27 | 92.48 | 0.21 | 40.81 | 22.12 | 45.80 | 0.27 | - | - |
| 2.2.3 | 2020 | PFP [37] | 91.40 | 90.91 | -0.49 | 40.81 | 22.26 | 45.46 | 0.27 | 0.10 | 62.67 |
| 2.6.2 | 2019 | TAS [88] | 92.88 | 92.88 | 0.00 | 40.81 | 22.45 | 45.00 | 0.27 | - | - |
| 2.7.3 | 2022 | GKP-TMI [89] | 92.35 | 92.01 | -0.34 | 40.81 | 23.30 | 42.90 | 0.27 | 0.15 | 43.40 |
| 2.5.2 | 2021 | DDG [83] | 92.24 | 92.27 | 0.03 | 40.81 | 23.38 | 42.70 | 0.27 | - | - |
| 2.5.1 | 2018 | SFP [90] | 92.20 | 90.83 | -1.37 | 40.81 | 23.59 | 42.20 | 0.27 | - | - |
| 2.2.1 | 2021 | LRMF [68] | 92.20 | 91.04 | -1.16 | 40.81 | 23.59 | 42.20 | 0.27 | - | - |
| 2.7.3 | 2022 | SOKS [54] | 92.05 | 91.83 | -0.22 | 40.81 | 23.63 | 42.09 | 0.27 | 0.16 | 40.74 |
| 2.2.1 | 2022 | GCNP [52] | 92.25 | 92.22 | -0.03 | 40.81 | 28.38 | 30.47 | 0.27 | 0.20 | 27.42 |
| 2.5.1 | 2018 | SFP [90] | 92.20 | 91.20 | -1.00 | 40.81 | 28.85 | 29.30 | 0.27 | - | - |
| 2.6.2 | 2020 | DSA [79] | 92.17 | 92.10 | -0.07 | 40.81 | 30.20 | 26.00 | 0.27 | - | - |
| 2.4.2 | 2019 | VP [65] | 92.01 | 91.66 | -0.35 | 40.81 | 34.39 | 15.73 | 0.27 | 0.22 | 19.05 |
| ResNet-32 | | | | | | | | | | | |
| 2.4.1 | 2019 | ED [72] | 95.30 | 93.05 | -2.25 | 69.12 | 3.64 | 94.74 | 0.47 | 0.02 | 96.05 |
| 2.4.1 | 2019 | ED [72] | 95.30 | 95.17 | -0.13 | 69.12 | 20.56 | 70.25 | 0.47 | 0.13 | 71.99 |
| 2.4.1 | 2022 | SOSP [75] | 95.30 | 95.22 | -0.08 | 69.12 | 22.22 | 67.85 | 0.47 | 0.13 | 72.85 |
| 2.4.1 | 2022 | SOSP [75] | 95.30 | 95.06 | -0.24 | 69.12 | 22.56 | 67.36 | 0.47 | 0.13 | 72.33 |
| 2.5.2 | 2021 | ManiDP [81] | 92.66 | 92.15 | -0.51 | 69.12 | 25.44 | 63.20 | 0.47 | - | - |
| 2.3.2 | 2020 | SCOP [80] | 92.66 | 92.13 | -0.53 | 69.12 | 30.55 | 55.80 | 0.47 | 0.21 | 56.20 |
| 2.7.3 | 2022 | SOKS [54] | 92.82 | 92.02 | -0.80 | 69.12 | 31.39 | 54.58 | 0.47 | 0.21 | 54.35 |
| 2.5.2 | 2021 | DDG [83] | 93.22 | 92.96 | -0.26 | 69.12 | 31.52 | 54.40 | 0.47 | - | - |
| 2.6.2 | 2022 | DAIS [84] | 92.92 | 93.49 | 0.57 | 69.12 | 31.86 | 53.90 | 0.47 | - | - |
| 2.1.2 | 2019 | COP [51] | 92.64 | 91.97 | -0.67 | 69.12 | 31.86 | 53.90 | 0.47 | 0.20 | 57.50 |
| 2.6.2 | 2022 | MFP [91] | 92.63 | 91.85 | -0.78 | 69.12 | 32.35 | 53.20 | 0.47 | - | - |
| 2.2.1 | 2021 | LRMF [68] | 92.63 | 92.08 | -0.55 | 69.12 | 32.35 | 53.20 | 0.47 | - | - |
| 2.2.1 | 2021 | LRMF [68] | 92.63 | 92.08 | -0.55 | 69.12 | 32.35 | 53.20 | 0.47 | - | - |
| 2.1.2 | 2019 | FPGM [82] | 92.63 | 92.82 | 0.19 | 69.12 | 32.35 | 53.20 | 0.47 | - | - |
| 2.6.2 | 2020 | LFPC [92] | 92.63 | 92.12 | -0.51 | 69.12 | 32.76 | 52.60 | 0.47 | - | - |
| 2.6.1 | 2022 | GNN-RL [85] | 92.63 | 92.58 | -0.05 | 69.12 | 33.87 | 51.00 | 0.47 | - | - |
| 2.5.1 | 2021 | DCP-CAC [76] | 92.36 | 92.21 | -0.15 | 69.12 | 34.49 | 50.10 | 0.47 | 0.25 | 47.83 |
| 2.6.1 | 2021 | AGMC [86] | 92.63 | 90.96 | -1.67 | 69.12 | 34.56 | 50.00 | 0.47 | - | - |
| 2.6.2 | 2019 | TAS [88] | 93.89 | 93.16 | -0.73 | 69.12 | 34.97 | 49.40 | 0.47 | - | - |
| 2.7.3 | 2022 | SOKS [54] | 92.82 | 92.44 | -0.38 | 69.12 | 36.74 | 46.85 | 0.47 | 0.27 | 43.48 |
| 2.3.2 | 2021 | ABP [39] | 92.63 | 92.55 | -0.08 | 69.12 | 37.12 | 46.30 | 0.47 | 0.27 | 43.60 |
| 2.5.2 | 2021 | DDG [83] | 93.22 | 93.21 | -0.01 | 69.12 | 39.12 | 43.40 | 0.47 | - | - |
| 2.7.3 | 2022 | GKP-TMI [89] | 92.82 | 93.04 | 0.22 | 69.12 | 39.33 | 43.10 | 0.47 | 0.27 | 43.40 |
| 2.5.1 | 2018 | SFP [90] | 92.63 | 90.08 | -2.55 | 69.12 | 40.44 | 41.50 | 0.47 | - | - |
| 2.5.1 | 2021 | DCP-CAC [76] | 92.36 | 92.85 | 0.49 | 69.12 | 48.35 | 30.04 | 0.47 | 0.35 | 26.09 |
| 2.5.1 | 2018 | SFP [90] | 92.63 | 90.63 | -2.00 | 69.12 | 49.21 | 28.80 | 0.47 | - | - |
| ResNet-44 | | | | | | | | | | | |
| 2.5.1 | 2021 | DCP-CAC [76] | 92.45 | 92.42 | -0.03 | 97.15 | 48.54 | 50.04 | 0.66 | 0.35 | 47.69 |
| 2.6.1 | 2021 | AGMC [86] | 93.10 | 92.28 | -0.82 | 97.15 | 48.58 | 50.00 | 0.66 | - | - |
| 2.5.1 | 2021 | DCP-CAC [76] | 92.45 | 93.26 | 0.81 | 97.15 | 67.98 | 30.03 | 0.66 | 0.46 | 30.77 |

TABLE 5: ResNet-20/32/44 on CIFAR-10.

| Section | Year | Method | Baseline Top-1 Acc.(%) | Pruned Top-1 Acc.(%) | Top-1 Acc. ↓(%) | Baseline FLOPs (M) | Pruned FLOPs (M) | FLOPs ↓(%) | Baseline Params (M) | Pruned Params (M) | Params ↓(%) |
|---|---|---|---|---|---|---|---|---|---|---|---|
| ResNet-56 | | | | | | | | | | | |
| 2.2.3 | 2020 | PFP [37] | 92.95 | 92.67 | -0.28 | 125.75 | 19.59 | 84.42 | 0.86 | 0.09 | 88.98 |
| 2.6.1 | 2022 | DECORE [35] | 93.26 | 90.85 | -2.41 | 125.75 | 23.27 | 81.50 | 0.86 | 0.13 | 84.71 |
| 2.3.2 | 2021 | ResRep [93] | 93.71 | 92.66 | 1.05 | 125.75 | 27.88 | 77.83 | 0.86 | - | - |
| 2.2.1 | 2022 | GCNP [52] | 93.72 | 92.75 | -0.97 | 125.75 | 28.65 | 77.22 | 0.86 | 0.25 | 70.50 |
| 2.7.2 | 2020 | Hinge [66] | 92.95 | 92.65 | -0.30 | 125.75 | 30.18 | 76.00 | 0.86 | 0.18 | 79.20 |
| 2.7.3 | 2020 | SWP [56] | 93.10 | 92.98 | -0.12 | 125.75 | 30.68 | 75.60 | 0.86 | 0.19 | 77.70 |
| 2.2.1 | 2020 | HRank [45] | 93.26 | 90.72 | -2.54 | 125.75 | 32.59 | 74.09 | 0.86 | 0.27 | 68.24 |
| 2.2.1 | 2021 | CHIP [42] | 93.26 | 92.05 | -1.21 | 125.75 | 34.83 | 72.30 | 0.86 | 0.24 | 71.80 |
| 2.6.2 | 2022 | DAIS [84] | 92.53 | 93.53 | 1.00 | 125.75 | 36.59 | 70.90 | 0.86 | - | - |
| 2.3.1 | 2019 | GBN [94] | - | - | 0.03 | 125.75 | 37.35 | 70.30 | 0.86 | 0.29 | 66.70 |
| 2.6.2 | 2020 | DSA [79] | 93.12 | 92.20 | -0.92 | 125.75 | 40.99 | 67.40 | 0.86 | - | - |
| 2.5.2 | 2022 | FTWT [53] | 93.66 | 92.63 | -1.03 | 125.75 | 42.75 | 66.00 | 0.86 | - | - |
| 2.3.2 | 2021 | GDP-Guo [57] | 93.90 | 93.55 | -0.35 | 125.75 | 43.21 | 65.64 | 0.86 | - | - |
| 2.4.3 | 2022 | EKG [95] | 93.84 | 93.69 | -0.15 | 125.75 | 43.87 | 65.11 | 0.86 | - | - |
| 2.6.3 | 2022 | CCEP [59] | 93.48 | 93.24 | -0.24 | 125.75 | 46.00 | 63.42 | 0.86 | - | - |
| 2.5.2 | 2021 | ManiDP [81] | 93.70 | 93.64 | -0.06 | 125.75 | 47.28 | 62.40 | 0.86 | - | - |
| 2.1.2 | 2022 | EPruner [47] | 93.26 | 93.18 | -0.08 | 125.75 | 48.63 | 61.33 | 0.86 | 0.39 | 54.12 |
| 2.4.3 | 2019 | C-SGD [96] | 93.39 | 93.44 | 0.05 | 125.75 | 49.23 | 60.85 | 0.86 | - | - |
| 2.3.3 | 2021 | GREG [97] | 93.36 | 93.36 | 0.00 | 125.75 | 49.32 | 60.78 | 0.86 | - | - |
| 2.3.3 | 2021 | GREG [97] | 93.36 | 93.18 | -0.18 | 125.75 | 49.32 | 60.78 | 0.86 | - | - |
| 2.3.2 | 2019 | GAL [63] | 93.26 | 91.58 | -1.68 | 125.75 | 50.09 | 60.16 | 0.86 | 0.29 | 65.88 |
| 2.3.2 | 2019 | GAL [63] | 93.26 | 90.36 | -2.90 | 125.75 | 50.09 | 60.16 | 0.86 | 0.29 | 65.88 |
| 2.3.1 | 2019 | GBN [94] | - | - | -0.33 | 125.75 | 50.17 | 60.10 | 0.86 | 0.40 | 53.50 |
| 2.7.2 | 2021 | EDP [40] | 93.61 | 93.61 | 0.00 | 125.75 | 53.18 | 57.71 | 0.86 | 0.39 | 54.18 |
| 2.1.2 | 2022 | CLR-RNF [49] | 93.26 | 93.27 | 0.01 | 125.75 | 53.70 | 57.30 | 0.86 | 0.38 | 55.50 |
| 2.3.2 | 2020 | SCOP [80] | 93.70 | 93.64 | -0.06 | 125.75 | 55.33 | 56.00 | 0.86 | 0.38 | 56.30 |
| 2.6.2 | 2021 | EE [61] | 93.62 | 93.68 | 0.06 | 125.75 | 55.33 | 56.00 | 0.86 | - | - |
| 2.3.2 | 2022 | WhiteBox [46] | 93.26 | 93.54 | 0.28 | 125.75 | 55.83 | 55.60 | 0.86 | - | - |
| 2.6.1 | 2022 | RL-MCTS [41] | 93.20 | 93.56 | 0.36 | 125.75 | 56.59 | 55.00 | 0.86 | - | - |
| 2.6.3 | 2020 | ABCPruner [50] | 93.26 | 93.23 | -0.03 | 125.75 | 57.68 | 54.13 | 0.86 | 0.39 | 54.12 |
| 2.6.1 | 2022 | GNN-RL [85] | 93.39 | 93.49 | 0.10 | 125.75 | 57.84 | 54.00 | 0.86 | - | - |
| 2.5.2 | 2022 | FTWT [53] | 93.66 | 92.28 | -1.38 | 125.75 | 57.84 | 54.00 | 0.86 | - | - |
| 2.1.2 | 2021 | SRR [87] | 93.38 | 93.75 | 0.37 | 125.75 | 58.10 | 53.80 | 0.86 | - | - |
| 2.3.2 | 2021 | GDP-Guo [57] | 93.90 | 93.97 | 0.07 | 125.75 | 58.66 | 53.35 | 0.86 | - | - |
| 2.3.2 | 2020 | LeGR [98] | 93.90 | 93.70 | -0.20 | 125.75 | 59.10 | 53.00 | 0.86 | - | - |
| 2.3.2 | 2021 | ResRep [93] | 93.71 | 93.71 | 0.00 | 125.75 | 59.22 | 52.91 | 0.86 | - | - |
| 2.6.2 | 2020 | LFPC [92] | 93.59 | 93.34 | -0.25 | 125.75 | 59.23 | 52.90 | 0.86 | - | - |
| 2.6.2 | 2020 | LFPC [92] | 93.59 | 93.24 | -0.35 | 125.75 | 59.23 | 52.90 | 0.86 | - | - |
| 2.6.2 | 2019 | TAS [88] | 94.46 | 93.69 | -0.77 | 125.75 | 59.48 | 52.70 | 0.86 | - | - |
| 2.6.2 | 2022 | MFP [91] | 93.59 | 93.56 | -0.03 | 125.75 | 59.61 | 52.60 | 0.86 | - | - |
| 2.6.2 | 2022 | MFP [91] | 93.59 | 92.76 | -0.83 | 125.75 | 59.61 | 52.60 | 0.86 | - | - |
| 2.5.1 | 2018 | SFP [90] | 93.59 | 93.35 | -0.24 | 125.75 | 59.61 | 52.60 | 0.86 | - | - |
| 2.5.1 | 2018 | SFP [90] | 93.59 | 92.26 | -1.33 | 125.75 | 59.61 | 52.60 | 0.86 | - | - |
| 2.4.1 | 2019 | CCP [99] | 93.50 | - | 0.08 | 125.75 | 59.61 | 52.60 | 0.86 | - | - |
| 2.2.1 | 2021 | LRMF [68] | 93.59 | 93.25 | -0.34 | 125.75 | 59.61 | 52.60 | 0.86 | - | - |
| 2.2.1 | 2021 | LRMF [68] | 93.59 | 93.29 | -0.30 | 125.75 | 59.61 | 52.60 | 0.86 | - | - |
| 2.1.2 | 2019 | FPGM [82] | 93.59 | 93.49 | -0.10 | 125.75 | 59.61 | 52.60 | 0.86 | - | - |
| 2.2.3 | 2022 | DLRFC [44] | 93.06 | 93.57 | -0.51 | 125.75 | 59.63 | 52.58 | 0.86 | 0.38 | 55.63 |
| 2.6.2 | 2020 | DSA [79] | 93.12 | 92.91 | -0.21 | 125.75 | 60.11 | 52.20 | 0.86 | - | - |
| 2.7.2 | 2021 | CC [60] | 93.33 | 93.64 | 0.31 | 125.75 | 60.36 | 52.00 | 0.86 | 0.45 | 48.24 |
| 2.7.3 | 2022 | SOKS [54] | 93.06 | 93.08 | 0.02 | 125.75 | 60.70 | 51.73 | 0.86 | 0.39 | 54.12 |
| 2.3.1 | 2020 | SCP [58] | 93.69 | 93.23 | 0.46 | 125.75 | 60.99 | 51.50 | 0.86 | 0.44 | 48.47 |
| 2.6.2 | 2022 | DDNP [100] | 93.62 | 93.83 | 0.21 | 125.75 | 61.62 | 51.00 | 0.86 | - | - |
| 2.3.1 | 2020 | EagleEye [101] | - | 94.66 | - | 125.75 | 62.23 | 50.51 | 0.86 | - | - |
| 2.5.1 | 2021 | DCP-CAC [76] | 92.88 | 93.10 | 0.22 | 125.75 | 62.82 | 50.04 | 0.86 | 0.44 | 49.41 |
| 2.2.1 | 2020 | HRank [45] | 93.26 | 93.17 | -0.09 | 125.75 | 62.85 | 50.02 | 0.86 | 0.50 | 42.35 |
| 2.3.2 | 2020 | DMC [102] | 93.62 | 93.69 | 0.07 | 125.75 | 62.88 | 50.00 | 0.86 | - | - |
| 2.6.1 | 2018 | AMC [103] | 92.80 | 90.10 | -2.70 | 125.75 | 62.88 | 50.00 | 0.86 | - | - |
| 2.4.3 | 2022 | EKG [95] | 93.84 | 94.09 | 0.25 | 125.75 | 62.88 | 50.00 | 0.86 | - | - |
| 2.6.1 | 2021 | AGMC [86] | 93.39 | 92.76 | -0.63 | 125.75 | 62.88 | 50.00 | 0.86 | - | - |
| 2.7.2 | 2020 | Hinge [66] | 92.95 | 93.69 | 0.74 | 125.75 | 62.88 | 50.00 | 0.86 | 0.42 | 51.27 |
| 2.6.1 | 2018 | AMC [103] | 92.80 | 91.90 | -0.90 | 125.75 | 62.88 | 50.00 | 0.86 | - | - |
| 2.4.3 | 2022 | RollBack [104] | - | 92.53 | - | 125.75 | 62.88 | 50.00 | 0.86 | - | - |
| 2.6.1 | 2022 | DECORE [35] | 93.26 | 93.26 | 0.00 | 125.75 | 63.06 | 49.85 | 0.86 | 0.44 | 49.41 |
| 2.2.3 | 2018 | DCP [74] | 93.80 | 93.49 | -0.31 | 125.75 | 63.19 | 49.75 | 0.86 | 0.44 | 49.24 |
| 2.7.1 | 2022 | RRCP [105] | - | 93.48 | - | 125.75 | 64.17 | 48.97 | 0.86 | 0.47 | 44.92 |
| 2.2.1 | 2022 | GCNP [52] | 93.72 | 93.85 | 0.13 | 125.75 | 65.00 | 48.31 | 0.86 | 0.56 | 35.01 |
| 2.5.1 | 2021 | SEP [73] | 93.04 | 93.85 | 0.81 | 125.75 | 65.99 | 47.52 | 0.86 | 0.62 | 27.91 |
| 2.2.1 | 2021 | CHIP [42] | 93.26 | 94.16 | 0.90 | 125.75 | 66.14 | 47.40 | 0.86 | 0.49 | 42.80 |
| 2.6.2 | 2020 | LFPC [92] | 93.59 | 93.72 | 0.13 | 125.75 | 66.52 | 47.10 | 0.86 | - | - |

Continue on the next page...

TABLE 6: ResNet-56 on CIFAR-10. (Part 1)

| Section | Year | Method | Baseline Top-1 Acc.(%) | Pruned Top-1 Acc.(%) | Top-1 Acc. ↓(%) | Baseline FLOPs (M) | Pruned FLOPs (M) | FLOPs ↓(%) | Baseline Params (M) | Pruned Params (M) | Params ↓(%) |
|---|---|---|---|---|---|---|---|---|---|---|---|
| ResNet-56 (cont.) | | | | | | | | | | | |
| 2.6.2 | 2020 | LFPC [92] | 93.59 | 93.56 | -0.03 | 125.75 | 66.52 | 47.10 | 0.86 | - | - |
| 2.2.3 | 2018 | DCP [74] | 93.80 | 93.81 | 0.01 | 125.75 | 66.53 | 47.09 | 0.86 | 0.26 | 70.33 |
| 2.4.1 | 2019 | CCP [99] | 93.50 | - | -0.19 | 125.75 | 66.65 | 47.00 | 0.86 | - | - |
| 2.3.1 | 2020 | PR [62] | 93.80 | 93.83 | -0.03 | 125.75 | 66.65 | 47.00 | 0.86 | - | - |
| 2.3.2 | 2021 | ABP [39] | 93.41 | 93.10 | -0.31 | 125.75 | 68.91 | 45.20 | 0.86 | 0.47 | 45.70 |
| 2.2.3 | 2018 | NISP [106] | - | - | 0.03 | 125.75 | 70.91 | 43.61 | 0.86 | 0.49 | 42.60 |
| 2.7.3 | 2022 | GKP-TMI [89] | 93.78 | 94.00 | 0.22 | 125.75 | 71.39 | 43.23 | 0.86 | 0.49 | 43.49 |
| 2.7.2 | 2021 | CC [60] | 93.33 | 93.87 | 0.54 | 125.75 | 72.43 | 42.40 | 0.86 | 0.55 | 36.47 |
| 2.5.1 | 2018 | SFP [90] | 93.59 | 93.78 | 0.19 | 125.75 | 74.07 | 41.10 | 0.86 | - | - |
| 2.5.1 | 2018 | SFP [90] | 93.59 | 93.10 | -0.49 | 125.75 | 74.07 | 41.10 | 0.86 | - | - |
| 2.4.1 | 2022 | HAP [107] | 93.88 | 93.55 | 0.33 | 125.75 | 74.57 | 40.70 | 0.86 | - | - |
| 2.3.2 | 2019 | GAL [63] | 93.26 | 93.38 | 0.12 | 125.75 | 78.46 | 37.60 | 0.86 | 0.76 | 11.76 |
| 2.3.2 | 2019 | GAL [63] | 93.26 | 92.98 | -0.28 | 125.75 | 78.46 | 37.60 | 0.86 | 0.76 | 11.76 |
| 2.7.3 | 2022 | SOKS [54] | 93.06 | 93.22 | 0.16 | 125.75 | 80.60 | 35.91 | 0.86 | 0.52 | 40.00 |
| 2.7.3 | 2019 | SDN [67] | 93.03 | 93.29 | 0.26 | 125.75 | 81.99 | 34.80 | 0.86 | 0.50 | 42.30 |
| 2.5.1 | 2021 | SEP [73] | 93.04 | 94.05 | 1.01 | 125.75 | 82.89 | 34.08 | 0.86 | 0.62 | 27.91 |
| 2.5.1 | 2021 | DCP-CAC [76] | 92.88 | 93.47 | 0.59 | 125.75 | 88.01 | 30.01 | 0.86 | 0.60 | 30.59 |
| 2.3.2 | 2020 | LeGR [98] | 93.90 | 94.10 | 0.20 | 125.75 | 88.02 | 30.00 | 0.86 | - | - |
| 2.2.1 | 2020 | HRank [45] | 93.26 | 93.52 | 0.26 | 125.75 | 88.90 | 29.30 | 0.86 | 0.72 | 16.47 |
| 2.6.2 | 2020 | DSA [79] | 93.12 | 93.08 | -0.04 | 125.75 | 88.91 | 29.30 | 0.86 | - | - |
| 2.1.1 | 2017 | PFEC [69] | 93.04 | 93.06 | 0.02 | 125.75 | 91.04 | 27.60 | 0.86 | 0.74 | 13.73 |
| 2.6.1 | 2022 | DECORE [35] | 93.26 | 93.34 | 0.08 | 125.75 | 92.67 | 26.30 | 0.86 | 0.65 | 24.71 |
| 2.4.1 | 2022 | HAP [107] | 93.88 | 92.92 | 0.96 | 125.75 | 95.70 | 23.90 | 0.86 | - | - |
| 2.4.2 | 2019 | VP [65] | 93.04 | 92.26 | -0.78 | 125.75 | 100.37 | 20.18 | 0.86 | 0.69 | 19.30 |
| 2.1.1 | 2017 | PFEC [69] | 93.04 | 93.10 | 0.06 | 125.75 | 112.67 | 10.40 | 0.86 | 0.78 | 9.41 |

TABLE 6: ResNet-56 on CIFAR-10. (Part 2)

| Section | Year | Method | Baseline Top-1 Acc.(%) | Pruned Top-1 Acc.(%) | Top-1 Acc. ↓(%) | Baseline FLOPs (M) | Pruned FLOPs (M) | FLOPs ↓(%) | Baseline Params (M) | Pruned Params (M) | Params ↓(%) |
|---|---|---|---|---|---|---|---|---|---|---|---|
| ResNet-110 | | | | | | | | | | | |
| 2.2.3 | 2020 | PFP [37] | 93.57 | 93.21 | -0.36 | 253.15 | 25.92 | 89.76 | 1.73 | 0.14 | 92.07 |
| 2.6.1 | 2022 | DECORE [35] | 93.50 | 92.71 | -0.79 | 253.15 | 58.43 | 76.92 | 1.73 | 0.35 | 79.65 |
| 2.2.1 | 2021 | CHIP [42] | 93.50 | 93.63 | 0.13 | 253.15 | 71.89 | 71.60 | 1.73 | 0.55 | 68.30 |
| 2.2.1 | 2020 | HRank [45] | 93.50 | 92.65 | -0.85 | 253.15 | 79.38 | 68.64 | 1.73 | 0.53 | 69.19 |
| 2.5.2 | 2021 | DDG [83] | 94.25 | 93.87 | -0.38 | 253.15 | 83.03 | 67.20 | 1.73 | - | - |
| 2.6.3 | 2022 | CCEP [59] | 93.68 | 93.46 | -0.22 | 253.15 | 83.31 | 67.09 | 1.73 | - | - |
| 2.3.2 | 2022 | WhiteBox [46] | 93.50 | 94.12 | 0.62 | 253.15 | 86.07 | 66.00 | 1.73 | - | - |
| 2.1.2 | 2022 | CLR-RNF [49] | 93.57 | 93.71 | 0.14 | 253.15 | 86.07 | 66.00 | 1.73 | 0.53 | 69.10 |
| 2.1.2 | 2022 | EPruner [47] | 93.50 | 93.62 | 0.12 | 253.15 | 86.31 | 65.91 | 1.73 | 0.41 | 76.30 |
| 2.6.3 | 2020 | ABCPruner [50] | 93.50 | 93.58 | 0.08 | 253.15 | 88.49 | 65.04 | 1.73 | 0.56 | 67.63 |
| 2.2.1 | 2021 | LRMF [68] | 93.68 | 93.61 | -0.07 | 253.15 | 94.17 | 62.80 | 1.73 | - | - |
| 2.6.2 | 2022 | MFP [91] | 93.68 | 93.38 | -0.30 | 253.15 | 94.17 | 62.80 | 1.73 | - | - |
| 2.6.1 | 2022 | DECORE [35] | 93.50 | 93.50 | 0.00 | 253.15 | 96.76 | 61.78 | 1.73 | 0.61 | 64.53 |
| 2.4.3 | 2019 | C-SGD [96] | 94.38 | 94.44 | 0.06 | 253.15 | 99.01 | 60.89 | 1.73 | - | - |
| 2.6.2 | 2020 | LFPC [92] | 93.68 | 93.07 | -0.61 | 253.15 | 100.50 | 60.30 | 1.73 | - | - |
| 2.6.2 | 2020 | LFPC [92] | 93.68 | 93.79 | 0.11 | 253.15 | 100.50 | 60.30 | 1.73 | - | - |
| 2.6.2 | 2022 | DAIS [84] | 95.62 | 95.02 | -0.60 | 253.15 | 101.26 | 60.00 | 1.73 | - | - |
| 2.3.2 | 2021 | ResRep [93] | 94.64 | 94.62 | 0.02 | 253.15 | 105.79 | 58.21 | 1.73 | - | - |
| 2.5.2 | 2021 | DDG [83] | 94.25 | 94.33 | 0.08 | 253.15 | 111.13 | 56.10 | 1.73 | - | - |
| 2.6.2 | 2022 | MFP [91] | 93.68 | 93.31 | -0.37 | 253.15 | 120.75 | 52.30 | 1.73 | - | - |
| 2.6.2 | 2022 | MFP [91] | 93.68 | 93.69 | 0.01 | 253.15 | 120.75 | 52.30 | 1.73 | - | - |
| 2.6.2 | 2019 | TAS [88] | 94.97 | 94.33 | -0.64 | 253.15 | 120.75 | 52.30 | 1.73 | - | - |
| 2.2.1 | 2021 | LRMF [68] | 93.68 | 93.88 | 0.20 | 253.15 | 120.75 | 52.30 | 1.73 | - | - |
| 2.1.2 | 2019 | FPGM [82] | 93.68 | 93.85 | 0.17 | 253.15 | 120.75 | 52.30 | 1.73 | - | - |
| 2.2.1 | 2021 | LRMF [68] | 93.68 | 93.73 | 0.05 | 253.15 | 120.75 | 52.30 | 1.73 | - | - |
| 2.2.1 | 2021 | CHIP [42] | 93.50 | 94.44 | 0.94 | 253.15 | 121.26 | 52.10 | 1.73 | 0.89 | 48.30 |
| 2.6.1 | 2022 | GNN-RL [85] | 93.68 | 94.31 | 0.63 | 253.15 | 121.51 | 52.00 | 1.73 | - | - |
| 2.5.1 | 2021 | DCP-CAC [76] | 93.38 | 93.86 | 0.48 | 253.15 | 126.52 | 50.02 | 1.73 | 0.89 | 48.84 |
| 2.6.1 | 2021 | AGMC [86] | 93.68 | 93.08 | -0.60 | 253.15 | 126.58 | 50.00 | 1.73 | - | - |
| 2.3.2 | 2019 | GAL [63] | 93.50 | 92.74 | -0.76 | 253.15 | 130.33 | 48.52 | 1.73 | 0.96 | 44.77 |
| 2.3.2 | 2019 | GAL [63] | 93.50 | 92.55 | -0.95 | 253.15 | 130.33 | 48.52 | 1.73 | 0.96 | 44.77 |
| 2.3.2 | 2021 | ABP [39] | 93.63 | 93.95 | 0.32 | 253.15 | 136.19 | 46.20 | 1.73 | 0.95 | 44.90 |
| 2.2.3 | 2018 | NISP [106] | - | - | 0.18 | 253.15 | 142.32 | 43.78 | 1.73 | 0.98 | 43.25 |
| 2.7.3 | 2022 | GKP-TMI [89] | 94.26 | 94.90 | 0.64 | 253.15 | 143.51 | 43.31 | 1.73 | 0.98 | 43.52 |
| 2.2.1 | 2020 | HRank [45] | 93.50 | 94.23 | 0.73 | 253.15 | 148.85 | 41.20 | 1.73 | 1.05 | 39.53 |
| 2.5.1 | 2018 | SFP [90] | 93.68 | 93.38 | -0.30 | 253.15 | 149.86 | 40.80 | 1.73 | - | - |
| 2.5.1 | 2018 | SFP [90] | 93.68 | 93.86 | 0.18 | 253.15 | 149.86 | 40.80 | 1.73 | - | - |
| 2.1.1 | 2017 | PFEC [69] | 93.53 | 93.30 | -0.23 | 253.15 | 155.43 | 38.60 | 1.73 | 1.17 | 32.40 |
| 2.4.2 | 2019 | VP [65] | 93.21 | 92.96 | -0.25 | 253.15 | 160.61 | 36.56 | 1.73 | 1.02 | 41.07 |
| 2.6.1 | 2022 | DECORE [35] | 93.50 | 93.88 | 0.38 | 253.15 | 163.47 | 35.43 | 1.73 | 1.12 | 35.47 |
| 2.5.1 | 2021 | DCP-CAC [76] | 93.38 | 94.11 | 0.73 | 253.15 | 176.97 | 30.09 | 1.73 | 1.23 | 29.07 |
| 2.5.1 | 2018 | SFP [90] | 93.68 | 93.93 | 0.25 | 253.15 | 181.76 | 28.20 | 1.73 | - | - |
| 2.3.2 | 2019 | GAL [63] | 93.50 | 93.59 | 0.09 | 253.15 | 205.91 | 18.66 | 1.73 | 1.66 | 4.07 |
| 2.3.2 | 2019 | GAL [63] | 93.50 | 92.55 | -0.95 | 253.15 | 205.91 | 18.66 | 1.73 | 1.66 | 4.07 |
| 2.1.1 | 2017 | PFEC [69] | 93.53 | 93.55 | 0.02 | 253.15 | 213.13 | 15.81 | 1.73 | 1.69 | 2.33 |
| ResNet-164 | | | | | | | | | | | |
| 2.4.3 | 2019 | C-SGD [96] | 94.83 | 94.75 | -0.08 | 247.65 | 96.81 | 60.91 | 1.70 | - | - |
| 2.7.2 | 2020 | Hinge [66] | 95.18 | 94.60 | -0.58 | 247.65 | 110.01 | 55.58 | 1.70 | 0.86 | 49.47 |
| 2.4.2 | 2019 | VP [65] | 93.58 | 93.16 | -0.42 | 247.65 | 126.21 | 49.04 | 1.70 | 0.74 | 56.55 |
| 2.3.1 | 2017 | NS [77] | 94.58 | 94.73 | 0.15 | 247.65 | 136.48 | 44.89 | 1.70 | 1.10 | 35.29 |
| 2.6.2 | 2019 | TAS [88] | 95.47 | 94.00 | -1.47 | 247.65 | 178.06 | 28.10 | 1.70 | - | - |
| 2.3.1 | 2017 | NS [77] | 94.58 | 94.92 | 0.34 | 247.65 | 189.09 | 23.65 | 1.70 | 1.44 | 15.29 |

TABLE 7: ResNet-110/164 on CIFAR-10.

| Section | Year | Method | Baseline Top-1 Acc.(%) | Pruned Top-1 Acc.(%) | Top-1 Acc. ↓(%) | Baseline FLOPs (M) | Pruned FLOPs (M) | FLOPs ↓(%) | Baseline Params (M) | Pruned Params (M) | Params ↓(%) |
|---|---|---|---|---|---|---|---|---|---|---|---|
| ResNet-18 | | | | | | | | | | | |
| 2.3.3 | 2019 | OICSR [108] | 94.46 | 92.44 | -2.02 | 557.21 | 30.65 | 94.50 | 11.17 | - | - |
| 2.4.3 | 2022 | StructADMM [36] | - | 93.80 | - | 557.21 | 45.67 | 91.80 | 11.17 | - | - |
| 2.6.1 | 2020 | AutoCompress [34] | 93.90 | 93.81 | -0.09 | 557.21 | 45.67 | 91.80 | 11.17 | - | - |
| 2.3.3 | 2019 | OICSR [108] | 94.46 | 94.27 | -0.19 | 557.21 | 75.22 | 86.50 | 11.17 | - | - |
| 2.6.2 | 2022 | DNCP [109] | 95.35 | 94.97 | -0.38 | 557.21 | 140.56 | 74.77 | 11.17 | - | - |
| 2.5.2 | 2022 | CDG [110] | 91.26 | 90.37 | -0.89 | 557.21 | 257.97 | 53.70 | 11.17 | - | - |
| 2.6.2 | 2022 | DNCP [109] | 95.35 | 95.31 | -0.04 | 557.21 | 314.25 | 43.60 | 11.17 | - | - |
| 2.3.3 | 2019 | OICSR [108] | 94.46 | 95.10 | 0.64 | 557.21 | 338.78 | 39.20 | 11.17 | - | - |
| 2.6.3 | 2022 | EDropout [111] | 92.81 | 90.96 | -1.85 | 557.21 | - | - | 11.17 | 5.49 | 50.89 |
| 2.7.1 | 2022 | EarlyCroP [70] | 91.50 | 91.00 | -0.50 | 557.21 | - | - | 11.17 | 0.55 | 95.10 |
| 2.7.3 | 2022 | DPP [71] | 93.60 | 93.14 | -0.46 | 557.21 | - | - | 11.17 | 4.13 | 63.06 |
| ResNet-34 | | | | | | | | | | | |
| 2.6.3 | 2022 | EDropout [111] | 92.80 | 88.21 | -4.59 | 1160 | - | - | 21.60 | 8.42 | 61.03 |
| ResNet-50 | | | | | | | | | | | |
| 2.3.3 | 2021 | OTO [38] | 93.50 | 94.40 | 0.90 | 1307 | 167.30 | 87.20 | 23.52 | 2.07 | 91.20 |
| 2.6.3 | 2022 | EDropout [111] | 92.21 | 85.30 | -6.91 | 1307 | - | - | 23.52 | 10.91 | 53.62 |
| ResNet-101 | | | | | | | | | | | |
| 2.7.1 | 2020 | EB [64] | - | 92.49 | - | 7595.00 | 3452.27 | 54.55 | 44.54 | 13.36 | 70.00 |
| 2.7.1 | 2020 | EB [64] | - | 93.90 | - | 7595.00 | 5425.00 | 28.57 | 44.54 | 22.27 | 50.00 |
| 2.7.1 | 2020 | EB [64] | - | 93.91 | - | 7595.00 | 6904.55 | 9.09 | 44.54 | 31.18 | 30.00 |
| 2.6.3 | 2022 | EDropout [111] | 92.66 | 86.57 | -6.09 | 2520.00 | - | - | 42.51 | 19.20 | 54.82 |

TABLE 8: ResNet-18/34/50/101 on CIFAR-10.

| Section | Year | Method | Baseline Top-1 Acc.(%) | Pruned Top-1 Acc.(%) | Top-1 Acc. ↓(%) | Baseline FLOPs (M) | Pruned FLOPs (M) | FLOPs ↓(%) | Baseline Params (M) | Pruned Params (M) | Params ↓(%) |
|---|---|---|---|---|---|---|---|---|---|---|---|
| MobileNet-V1 | | | | | | | | | | | |
| 2.3.1 | 2020 | EagleEye [101] | - | 88.01 | - | 34.20 | 3.30 | 90.35 | 4.20 | - | - |
| 2.5.2 | 2022 | FTWT [53] | 90.89 | 91.21 | 0.32 | 34.20 | 7.52 | 78.00 | 4.20 | - | - |
| 2.6.2 | 2022 | DAIS [84] | 90.87 | 91.87 | 1.00 | 34.20 | 11.42 | 66.60 | 4.20 | - | - |
| 2.3.1 | 2020 | EagleEye [101] | - | 91.44 | - | 34.20 | 12.10 | 64.62 | 4.20 | - | - |
| 2.2.3 | 2018 | DCP [74] | 93.96 | 94.37 | 0.41 | 34.20 | 19.54 | 42.86 | 4.20 | 2.94 | 30.07 |
| 2.3.1 | 2020 | EagleEye [101] | - | 91.89 | - | 34.20 | 26.50 | 22.51 | 4.20 | - | - |
| 2.7.3 | 2022 | DPP [71] | 93.78 | 93.96 | 0.18 | 34.20 | - | - | 4.20 | 1.57 | 62.70 |
| MobileNet-V2 | | | | | | | | | | | |
| 2.4.3 | 2022 | StructADMM [36] | - | 95.10 | - | 89.00 | 22.82 | 74.36 | 3.50 | - | - |
| 2.6.2 | 2022 | DNCP [109] | 94.15 | 93.30 | -0.85 | 89.00 | 25.00 | 71.91 | 3.50 | - | - |
| 2.4.3 | 2022 | EKG [95] | 94.21 | 94.52 | 0.31 | 89.00 | 44.50 | 50.00 | 3.50 | - | - |
| 2.3.2 | 2021 | GDP-Guo [57] | 94.89 | 95.15 | 0.26 | 89.00 | 47.86 | 46.22 | 3.50 | - | - |
| 2.6.2 | 2022 | DDNP [100] | 94.58 | 94.81 | 0.23 | 89.00 | 50.73 | 43.00 | 3.50 | - | - |
| 2.6.2 | 2022 | DNCP [109] | 94.15 | 93.71 | -0.44 | 89.00 | 52.00 | 41.57 | 3.50 | - | - |
| 2.3.2 | 2020 | SCOP [80] | 94.48 | 94.24 | -0.24 | 89.00 | 53.13 | 40.30 | 3.50 | 2.24 | 36.10 |
| 2.3.2 | 2020 | DMC [102] | 94.23 | 94.49 | 0.26 | 89.00 | 53.40 | 40.00 | 3.50 | - | - |
| 2.3.2 | 2022 | WhiteBox [46] | 95.02 | 95.28 | 0.26 | 89.00 | 63.01 | 29.20 | 3.50 | - | - |
| 2.2.3 | 2018 | DCP [74] | 94.47 | 94.69 | 0.22 | 89.00 | 65.44 | 26.47 | 3.50 | 2.67 | 23.66 |

TABLE 9: MobileNet-V1/V2 on CIFAR-10.

| Section | Year | Method | Baseline Top-1 Acc.(%) | Pruned Top-1 Acc.(%) | Top-1 Acc. ↓(%) | Baseline FLOPs (M) | Pruned FLOPs (M) | FLOPs ↓(%) | Baseline Params (M) | Pruned Params (M) | Params ↓(%) |
|---|---|---|---|---|---|---|---|---|---|---|---|
| DenseNet-40 | | | | | | | | | | | |
| 2.3.2 | 2019 | GAL [63] | 94.81 | 93.23 | -1.58 | 283.00 | 80.91 | 71.41 | 1.04 | 0.26 | 75.00 |
| 2.3.2 | 2019 | GAL [63] | 94.81 | 91.90 | -2.91 | 283.00 | 80.91 | 71.41 | 1.04 | 0.26 | 75.00 |
| 2.3.1 | 2020 | SCP [58] | 94.39 | 93.77 | 0.62 | 283.00 | 82.72 | 70.77 | 1.04 | 0.26 | 75.41 |
| 2.2.1 | 2020 | HRank [45] | 94.81 | 93.68 | -1.13 | 283.00 | 110.54 | 60.94 | 1.04 | 0.48 | 53.85 |
| 2.7.2 | 2021 | CC [60] | 94.81 | 94.40 | -0.41 | 283.00 | 112.00 | 60.42 | 1.04 | 0.37 | 64.42 |
| 2.4.3 | 2019 | C-SGD [96] | 93.81 | 94.44 | 0.63 | 283.00 | 113.06 | 60.05 | 1.04 | - | - |
| 2.3.1 | 2017 | NS [77] | 93.89 | 94.35 | 0.46 | 283.00 | 127.43 | 54.97 | 1.04 | 0.36 | 65.69 |
| 2.3.2 | 2019 | GAL [63] | 94.81 | 94.50 | -0.31 | 283.00 | 128.15 | 54.72 | 1.04 | 0.45 | 56.73 |
| 2.3.2 | 2019 | GAL [63] | 94.81 | 93.53 | -1.28 | 283.00 | 128.15 | 54.72 | 1.04 | 0.45 | 56.73 |
| 2.6.1 | 2022 | DECORE [35] | 94.81 | 94.04 | -0.77 | 283.00 | 128.17 | 54.71 | 1.04 | 0.37 | 64.42 |
| 2.7.2 | 2021 | CC [60] | 94.81 | 94.67 | -0.14 | 283.00 | 150.00 | 47.00 | 1.04 | 0.50 | 51.92 |
| 2.4.2 | 2019 | VP [65] | 94.11 | 93.16 | -0.95 | 283.00 | 156.55 | 44.68 | 1.04 | 0.42 | 59.62 |
| 2.7.2 | 2020 | Hinge [66] | 94.74 | 94.67 | -0.07 | 283.00 | 157.35 | 44.40 | 1.04 | 0.75 | 27.54 |
| 2.2.1 | 2020 | HRank [45] | 94.81 | 94.24 | -0.57 | 283.00 | 168.00 | 40.63 | 1.04 | 0.66 | 36.54 |
| 2.6.1 | 2022 | DECORE [35] | 94.81 | 94.59 | -0.22 | 283.00 | 171.41 | 39.43 | 1.04 | 0.56 | 46.15 |
| 2.3.2 | 2019 | GAL [63] | 94.81 | 94.61 | -0.20 | 283.00 | 182.97 | 35.35 | 1.04 | 0.67 | 35.58 |
| 2.3.2 | 2019 | GAL [63] | 94.81 | 94.29 | -0.52 | 283.00 | 182.97 | 35.35 | 1.04 | 0.67 | 35.58 |
| 2.3.1 | 2017 | NS [77] | 93.89 | 94.81 | 0.92 | 283.00 | 202.29 | 28.52 | 1.04 | 0.67 | 35.29 |
| 2.4.1 | 2022 | SOSP [75] | 94.58 | 94.41 | -0.17 | 283.00 | 209.02 | 26.14 | 1.04 | 0.68 | 34.78 |
| 2.4.1 | 2022 | SOSP [75] | 94.58 | 94.42 | -0.16 | 283.00 | 220.66 | 22.03 | 1.04 | 0.71 | 32.21 |
| 2.6.1 | 2022 | DECORE [35] | 94.81 | 94.85 | 0.04 | 283.00 | 229.02 | 19.07 | 1.04 | 0.83 | 20.19 |
| GoogLeNet | | | | | | | | | | | |
| 2.6.1 | 2022 | DECORE [35] | 95.05 | 94.33 | -0.72 | 1535.00 | 232.27 | 84.87 | 6.17 | 0.86 | 86.02 |
| 2.6.1 | 2022 | DECORE [35] | 95.05 | 94.51 | -0.54 | 1535.00 | 333.26 | 78.29 | 6.17 | 1.17 | 80.98 |
| 2.2.1 | 2020 | HRank [45] | 95.05 | 94.07 | -0.98 | 1535.00 | 454.44 | 70.39 | 6.17 | 1.87 | 69.76 |
| 2.1.2 | 2022 | CLR-RNF [49] | 95.03 | 94.85 | -0.18 | 1535.00 | 492.73 | 67.90 | 6.17 | 2.18 | 64.70 |
| 2.1.2 | 2022 | EPruner [47] | 95.05 | 94.99 | -0.06 | 1535.00 | 501.02 | 67.36 | 6.17 | 2.22 | 64.02 |
| 2.6.3 | 2020 | ABCPruner [50] | 95.05 | 94.84 | -0.21 | 1535.00 | 513.34 | 66.56 | 6.17 | 2.46 | 60.13 |
| 2.7.2 | 2021 | CC [60] | 95.05 | 94.88 | -0.17 | 1535.00 | 616.02 | 59.87 | 6.17 | 2.27 | 63.25 |
| 2.2.1 | 2020 | HRank [45] | 95.05 | 94.53 | -0.52 | 1535.00 | 696.81 | 54.61 | 6.17 | 2.75 | 55.45 |
| 2.7.2 | 2021 | CC [60] | 95.05 | 95.18 | 0.13 | 1535.00 | 767.50 | 50.00 | 6.17 | 2.84 | 53.98 |
| 2.3.2 | 2019 | GAL [63] | 95.05 | 93.93 | -1.12 | 1535.00 | 949.28 | 38.16 | 6.17 | 3.13 | 49.27 |
| 2.3.2 | 2019 | GAL [63] | 95.05 | 94.56 | -0.49 | 1535.00 | 949.28 | 38.16 | 6.17 | 3.13 | 49.27 |
| 2.6.1 | 2022 | DECORE [35] | 95.05 | 95.20 | 0.15 | 1535.00 | 1232.04 | 19.74 | 6.17 | 4.75 | 23.09 |
| PreResNet-29 | | | | | | | | | | | |
| 2.4.1 | 2019 | ED [72] | 94.42 | 89.10 | -5.32 | 41.28 | 3.85 | 90.67 | 0.27 | 0.02 | 93.45 |
| 2.4.1 | 2019 | ED [72] | 94.42 | 93.80 | -0.62 | 41.28 | 15.22 | 63.13 | 0.27 | 0.08 | 70.09 |
| PreResNet-101 | | | | | | | | | | | |
| 2.7.1 | 2020 | EB [64] | - | 92.49 | - | 7595.00 | 3452.27 | 54.55 | 44.54 | 13.36 | 70.00 |
| 2.7.1 | 2020 | EB [64] | - | 93.90 | - | 7595.00 | 5425.00 | 28.57 | 44.54 | 22.27 | 50.00 |
| 2.7.1 | 2020 | EB [64] | - | 93.91 | - | 7595.00 | 6904.55 | 9.09 | 44.54 | 31.18 | 30.00 |
| ResNeXt-20 | | | | | | | | | | | |
| 2.7.2 | 2020 | Hinge [66] | 92.54 | 91.96 | -0.58 | 36.00 | 21.24 | 41.00 | 0.21 | 0.13 | 36.05 |
| ResNeXt-164 | | | | | | | | | | | |
| 2.7.2 | 2020 | Hinge [66] | 95.18 | 94.87 | -0.31 | 210.00 | 93.28 | 55.58 | 1.70 | 0.86 | 49.47 |
| NAS | | | | | | | | | | | |
| 2.6.2 | 2022 | ReCNAS [112] | - | 97.48 | - | - | 300 | - | - | 4.10 | - |
| 2.6.2 | 2022 | ReCNAS [112] | - | 97.71 | - | - | 500 | - | - | 5.20 | - |

TABLE 10: Other models on CIFAR-10, including DenseNet-40, GoogLeNet, PreResNet-29/101, ResNeXt-20/164, and models searched by Neural Architecture Search (NAS).

| Section | Year | Method | Baseline Top-1 Acc.(%) | Pruned Top-1 Acc.(%) | Top-1 Acc. ↓(%) | Baseline FLOPs (M) | Pruned FLOPs (M) | FLOPs ↓(%) | Baseline Params (M) | Pruned Params (M) | Params ↓(%) |
|---|---|---|---|---|---|---|---|---|---|---|---|
| VGG-16 | | | | | | | | | | | |
| 2.3.1 | 2020 | SCP [58] | 73.51 | 69.96 | 3.55 | 314.59 | 65.31 | 79.24 | 14.73 | 0.88 | 94.01 |
| 2.2.1 | 2022 | GCNP [52] | 72.00 | 71.64 | -0.36 | 314.59 | 99.91 | 68.24 | 14.73 | 1.70 | 88.46 |
| 2.2.1 | 2022 | GCNP [52] | 72.00 | 72.00 | 0.00 | 314.59 | 136.59 | 56.58 | 14.73 | 2.87 | 80.49 |
| 2.3.1 | 2020 | SCP [58] | 73.51 | 73.86 | -0.35 | 314.59 | 152.73 | 51.45 | 14.73 | 2.93 | 80.14 |
| 2.2.3 | 2022 | DLRFC [44] | 73.54 | 74.09 | -0.55 | 314.59 | 178.06 | 43.40 | 14.73 | 2.58 | 82.50 |
| 2.1.2 | 2019 | COP [51] | 72.59 | 71.77 | -0.82 | 314.59 | 179.00 | 43.10 | 14.73 | 3.95 | 73.20 |
| 2.3.1 | 2020 | PR [62] | 73.83 | 74.25 | -0.42 | 314.59 | 179.32 | 43.00 | 14.73 | - | - |
| 2.2.1 | 2021 | LRMF [68] | - | - | 0.50 | 314.59 | 201.65 | 35.90 | 14.73 | - | - |
| 2.7.1 | 2020 | EB [64] | - | 71.28 | - | 314.59 | 209.73 | 33.33 | 14.73 | 7.37 | 50.00 |
| 2.7.3 | 2019 | SDN [67] | 72.38 | 73.43 | 1.05 | 314.59 | 211.09 | 32.90 | 14.73 | 3.11 | 78.90 |
| 2.4.2 | 2019 | VP [65] | 73.26 | 73.33 | 0.07 | 314.59 | 257.30 | 18.21 | 14.73 | 9.15 | 37.87 |
| 2.7.1 | 2020 | EB [64] | - | 72.17 | - | 314.59 | 262.16 | 16.67 | 14.73 | 10.31 | 30.00 |
| 2.7.1 | 2020 | EB [64] | - | 71.81 | - | 314.59 | 285.99 | 9.09 | 14.73 | 13.26 | 10.00 |
| 2.7.1 | 2022 | EarlyCroP [70] | - | 62.20 | - | 314.59 | - | - | 14.73 | 0.31 | 97.90 |
| 2.7.3 | 2022 | DPP [71] | 70.32 | 70.40 | 0.08 | 314.59 | - | - | 14.73 | 2.77 | 81.20 |
| VGG-19 | | | | | | | | | | | |
| 2.3.3 | 2021 | GREG [97] | 74.02 | 67.55 | -6.47 | 398.00.00 | 45.01 | 88.69 | 20.04 | - | - |
| 2.3.3 | 2021 | GREG [97] | 74.02 | 67.75 | -6.27 | 398.00 | 45.01 | 88.69 | 20.04 | - | - |
| 2.4.1 | 2019 | ED [72] | 73.08 | 64.91 | -8.17 | 398.00 | 45.17 | 88.65 | 20.04 | - | - |
| 2.4.1 | 2019 | ED [72] | 73.34 | 65.18 | -8.16 | 398.00 | 45.25 | 88.63 | 20.04 | - | - |
| 2.5.1 | 2021 | SEP [73] | 73.16 | 73.47 | 0.31 | 398.00 | 117.00 | 70.60 | 20.04 | 5.95 | 70.31 |
| 2.3.1 | 2020 | SCP [58] | 72.56 | 72.15 | 0.41 | 398.00 | 151.48 | 61.94 | 20.04 | 2.13 | 89.37 |
| 2.4.1 | 2022 | SOSP [75] | 73.45 | 73.11 | -0.34 | 398.00 | 192.59 | 51.61 | 20.04 | - | - |
| 2.4.1 | 2022 | SOSP [75] | 73.45 | 73.17 | -0.28 | 398.00 | 219.42 | 44.87 | 20.04 | - | - |
| 2.3.1 | 2020 | SCP [58] | 72.56 | 72.99 | -0.43 | 398.00 | 235.14 | 40.92 | 20.04 | 4.50 | 77.52 |
| 2.4.1 | 2019 | ED [72] | 73.08 | 73.01 | -0.07 | 398.00 | 248.91 | 37.46 | 20.04 | - | - |
| 2.4.1 | 2019 | ED [72] | 73.34 | 72.90 | -0.44 | 398.00 | 249.15 | 37.40 | 20.04 | - | - |
| 2.3.1 | 2017 | NS [77] | 73.26 | 73.48 | 0.22 | 398.00 | 250.19 | 37.14 | 20.04 | 4.99 | 75.10 |
| 2.5.1 | 2021 | DCP-CAC [76] | 70.17 | 72.28 | 2.11 | 398.00 | 251.00 | 36.93 | 20.04 | 8.93 | 55.44 |
| 2.7.1 | 2022 | ProsPr [78] | 72.50 | 72.29 | -0.21 | 398.00 | - | - | 20.04 | 4.01 | 80.00 |
| 2.7.1 | 2022 | ProsPr [78] | 73.50 | 71.12 | -2.38 | 398.00 | - | - | 20.04 | 2.00 | 90.00 |
| 2.7.1 | 2022 | ProsPr [78] | 74.50 | 68.03 | -6.47 | 398.00 | - | - | 20.04 | 1.00 | 95.00 |

TABLE 11: VGG-16/19 on CIFAR-100.

| Section | Year | Method | Baseline Top-1 Acc.(%) | Pruned Top-1 Acc.(%) | Top-1 Acc. ↓(%) | Baseline FLOPs (M) | Pruned FLOPs (M) | FLOPs ↓(%) | Baseline Params (M) | Pruned Params (M) | Params ↓(%) |
|---|---|---|---|---|---|---|---|---|---|---|---|
| ResNet-20 | | | | | | | | | | | |
| 2.7.2 | 2020 | Hinge [66] | 68.83 | 66.34 | -2.49 | 40.81 | 13.44 | 67.06 | 0.27 | 0.09 | 66.36 |
| 2.2.1 | 2022 | GCNP [52] | 68.38 | 66.14 | -2.24 | 40.81 | 16.38 | 59.87 | 0.27 | 0.14 | 49.42 |
| 2.6.2 | 2019 | TAS [88] | 68.69 | 68.90 | 0.21 | 40.81 | 22.45 | 45.00 | 0.27 | - | - |
| 2.2.1 | 2022 | GCNP [52] | 68.38 | 68.95 | 0.57 | 40.81 | 34.84 | 14.64 | 0.27 | 0.25 | 8.16 |
| ResNet-32 | | | | | | | | | | | |
| 2.4.1 | 2019 | ED [72] | 78.17 | 65.72 | -12.45 | 69.12 | 3.72 | 94.62 | 0.47 | - | - |
| 2.4.1 | 2022 | SOSP [75] | 76.80 | 75.33 | -1.47 | 69.12 | 17.78 | 74.28 | 0.47 | - | - |
| 2.4.1 | 2019 | ED [72] | 78.17 | 75.51 | -2.66 | 69.12 | 19.62 | 71.62 | 0.47 | - | - |
| 2.4.1 | 2022 | SOSP [75] | 76.80 | 75.52 | -1.28 | 69.12 | 19.63 | 71.60 | 0.47 | - | - |
| 2.5.1 | 2021 | DCP-CAC [76] | 68.48 | 68.11 | -0.37 | 69.12 | 34.49 | 50.10 | 0.47 | 0.25 | 47.83 |
| 2.6.2 | 2022 | DAIS [84] | 73.24 | 72.20 | -1.04 | 69.12 | 39.47 | 42.90 | 0.47 | - | - |
| 2.6.2 | 2019 | TAS [88] | 70.61 | 72.41 | 1.80 | 69.12 | 42.51 | 38.50 | 0.47 | - | - |
| 2.1.2 | 2019 | COP [51] | 68.74 | 68.29 | -0.45 | 69.12 | 45.48 | 34.20 | 0.47 | 0.30 | 35.20 |
| 2.5.1 | 2021 | DCP-CAC [76] | 68.48 | 69.51 | 1.03 | 69.12 | 48.35 | 30.04 | 0.47 | 0.35 | 26.09 |
| ResNet-44 | | | | | | | | | | | |
| 2.5.1 | 2021 | DCP-CAC [76] | 69.87 | 69.82 | -0.05 | 97.15 | 48.54 | 50.04 | 0.66 | 0.35 | 47.69 |
| 2.5.1 | 2021 | DCP-CAC [76] | 69.87 | 70.85 | 0.98 | 97.15 | 67.97 | 30.04 | 0.66 | 0.46 | 30.77 |
| ResNet-56 | | | | | | | | | | | |
| 2.3.3 | 2019 | OICSR [108] | 75.87 | 73.10 | -2.77 | 125.75 | 3.52 | 97.20 | 0.86 | - | - |
| 2.3.3 | 2019 | OICSR [108] | 75.87 | 75.75 | -0.12 | 125.75 | 17.35 | 86.20 | 0.86 | - | - |
| 2.6.2 | 2022 | DAIS [84] | 71.76 | 72.57 | 0.81 | 125.75 | 58.35 | 53.60 | 0.86 | - | - |
| 2.2.1 | 2021 | LRMF [68] | - | - | -0.44 | 125.75 | 59.61 | 52.60 | 0.86 | - | - |
| 2.2.1 | 2022 | GCNP [52] | 72.86 | 72.22 | -0.64 | 125.75 | 60.08 | 52.22 | 0.86 | 0.52 | 39.83 |
| 2.6.2 | 2020 | LFPC [92] | 70.25 | 70.83 | 0.58 | 125.75 | 60.86 | 51.60 | 0.86 | - | - |
| 2.6.2 | 2019 | TAS [88] | 73.18 | 72.25 | -0.93 | 125.75 | 61.24 | 51.30 | 0.86 | - | - |
| 2.5.1 | 2021 | DCP-CAC [76] | 70.90 | 70.10 | -0.80 | 125.75 | 62.82 | 50.04 | 0.86 | 0.44 | 49.41 |
| 2.4.2 | 2022 | EKG [95] | 72.62 | 72.93 | 0.31 | 125.75 | 62.88 | 50.00 | 0.86 | - | - |
| 2.2.1 | 2022 | GCNP [52] | 72.86 | 72.86 | 0.00 | 125.75 | 64.42 | 48.77 | 0.86 | 0.52 | 39.24 |
| 2.3.3 | 2019 | OICSR [108] | 75.87 | 76.23 | 0.36 | 125.75 | 77.34 | 38.50 | 0.86 | - | - |
| 2.7.3 | 2019 | SDN [67] | 70.01 | 69.78 | -0.23 | 125.75 | 77.59 | 38.30 | 0.86 | 0.55 | 36.10 |
| 2.5.1 | 2021 | DCP-CAC [76] | 70.90 | 71.31 | 0.41 | 125.75 | 88.01 | 30.01 | 0.86 | 0.60 | 30.59 |
| 2.2.3 | 2022 | DLRFC [44] | 71.14 | 71.41 | -0.27 | 125.75 | 93.68 | 25.50 | 0.86 | 0.64 | 25.90 |
| 2.3.1 | 2020 | PR [62] | 72.49 | 72.46 | 0.06 | 125.75 | 94.31 | 25.00 | 0.86 | - | - |
| ResNet-110 | | | | | | | | | | | |
| 2.6.2 | 2022 | DAIS [84] | 75.34 | 74.69 | -0.65 | 253.15 | 109.61 | 56.70 | 1.73 | - | - |
| 2.6.2 | 2019 | TAS [88] | 75.06 | 73.16 | -1.90 | 253.15 | 119.99 | 52.60 | 1.73 | - | - |
| 2.5.1 | 2021 | DCP-CAC [76] | 72.53 | 72.16 | -0.37 | 253.15 | 126.52 | 50.02 | 1.73 | 0.89 | 48.84 |
| 2.5.1 | 2021 | DCP-CAC [76] | 72.53 | 72.79 | 0.26 | 253.15 | 176.97 | 30.09 | 1.73 | 1.23 | 29.07 |
| ResNet-164 | | | | | | | | | | | |
| 2.3.1 | 2020 | SCP [58] | 77.24 | 75.05 | 2.19 | 247.65 | 86.85 | 64.93 | 1.70 | 0.79 | 53.30 |
| 2.3.1 | 2017 | NS [77] | 76.63 | 76.09 | -0.54 | 247.65 | 122.34 | 50.60 | 1.70 | 1.19 | 30.06 |
| 2.3.1 | 2020 | SCP [58] | 77.24 | 76.62 | 0.62 | 247.65 | 135.32 | 45.36 | 1.70 | 1.21 | 28.89 |
| 2.7.2 | 2020 | Hinge [66] | 76.78 | 76.88 | 0.10 | 247.65 | 137.00 | 44.68 | 1.70 | 1.30 | 23.43 |
| 2.3.1 | 2017 | NS [77] | 76.63 | 77.13 | 0.50 | 247.65 | 164.93 | 33.40 | 1.70 | 1.43 | 15.61 |
| 2.6.2 | 2019 | TAS [88] | 78.29 | 77.76 | -0.53 | 247.65 | 171.13 | 30.90 | 1.70 | - | - |
| 2.4.2 | 2019 | VP [65] | 75.56 | 73.76 | -1.80 | 247.65 | 180.18 | 27.24 | 1.70 | 1.40 | 17.86 |

TABLE 12: ResNet-20/32/44/56/110/164 on CIFAR-100.

| Section | Year | Method | Baseline Top-1 Acc.(%) | Pruned Top-1 Acc.(%) | Top-1 Acc. ↓(%) | Baseline FLOPs (M) | Pruned FLOPs (M) | FLOPs ↓(%) | Baseline Params (M) | Pruned Params (M) | Params ↓(%) |
|---|---|---|---|---|---|---|---|---|---|---|---|
| ResNet-18 | | | | | | | | | | | |
| 2.5.2 | 2022 | CDG [110] | 67.78 | 65.94 | -1.84 | 557.21 | 293.27 | 47.37 | 11.17 | - | - |
| 2.6.3 | 2022 | EDropout [111] | 69.03 | 67.06 | -1.97 | 557.21 | - | - | 11.17 | 5.39 | 51.79 |
| ResNet-34 | | | | | | | | | | | |
| 2.6.3 | 2022 | EDropout [111] | 69.96 | 64.79 | -5.17 | 1160.00 | - | - | 21.60 | 10.65 | 50.70 |
| ResNet-50 | | | | | | | | | | | |
| 2.6.2 | 2022 | DNCP [109] | 79.01 | 79.22 | 0.21 | 1307.00 | 739.62 | 43.41 | 23.52 | - | - |
| 2.6.3 | 2022 | EDropout [111] | 71.22 | 61.91 | -9.31 | 1307.00 | - | - | 23.52 | 10.82 | 54.01 |
| ResNet-101 | | | | | | | | | | | |
| 2.7.1 | 2020 | EB [64] | - | 72.29 | - | 7595.00 | 3038.00 | 60.00 | 44.54 | 13.36 | 70.00 |
| 2.7.1 | 2020 | EB [64] | - | 73.15 | - | 7595.00 | 5425.00 | 28.57 | 44.54 | 22.27 | 50.00 |
| 2.7.1 | 2020 | EB [64] | - | 73.52 | - | 7595.00 | 6329.17 | 16.67 | 44.54 | 31.18 | 30.00 |
| 2.6.3 | 2022 | EDropout [111] | 71.19 | 61.92 | -9.27 | 2520.00 | - | - | 42.51 | 18.56 | 56.34 |

TABLE 13: ResNet-18/34/50/101 on CIFAR-100.

| Section | Year | Method | Baseline Top-1 Acc.(%) | Pruned Top-1 Acc.(%) | Top-1 Acc. ↓(%) | Baseline FLOPs (M) | Pruned FLOPs (M) | FLOPs ↓(%) | Baseline Params (M) | Pruned Params (M) | Params ↓(%) |
|---|---|---|---|---|---|---|---|---|---|---|---|
| MobileNet-V1 | | | | | | | | | | | |
| 2.7.3 | 2022 | DPP [71] | 72.35 | 72.50 | -0.15 | - | - | - | - | - | 60 |
| MobileNet-V2 | | | | | | | | | | | |
| 2.4.2 | 2022 | EKG [95] | 76.07 | 76.29 | 0.22 | 89.00 | 44.50 | 50.00 | 3.50 | - | - |
| 2.6.2 | 2022 | DNCP [109] | 75.91 | 75.69 | -0.22 | 89.00 | 52.00 | 41.57 | 3.50 | - | - |

TABLE 14: MobileNet-V1/V2 on CIFAR-100.

| Section | Year | Method | Baseline Top-1 Acc.(%) | Pruned Top-1 Acc.(%) | Top-1 Acc. ↓(%) | Baseline FLOPs (M) | Pruned FLOPs (M) | FLOPs ↓(%) | Baseline Params (M) | Pruned Params (M) | Params ↓(%) |
|---|---|---|---|---|---|---|---|---|---|---|---|
| DenseNet-40 | | | | | | | | | | | |
| 2.3.1 | 2020 | SCP [58] | 74.24 | 73.17 | 1.07 | 283.00 | 91.07 | 67.82 | 1.04 | 0.26 | 74.86 |
| 2.3.1 | 2017 | NS [77] | 74.64 | 74.28 | -0.36 | 283.00 | 149.20 | 47.28 | 1.04 | 0.45 | 56.60 |
| 2.3.1 | 2020 | SCP [58] | 74.24 | 73.84 | 0.40 | 283.00 | 152.11 | 46.25 | 1.04 | 0.47 | 55.22 |
| 2.3.1 | 2017 | NS [77] | 74.64 | 74.72 | 0.08 | 283.00 | 196.98 | 30.39 | 1.04 | 0.65 | 37.74 |
| 2.4.1 | 2022 | SOSP [75] | 74.11 | 73.46 | -0.65 | 283.00 | 198.16 | 29.98 | 1.04 | - | - |
| 2.4.1 | 2022 | SOSP [75] | 74.11 | 73.60 | -0.51 | 283.00 | 203.11 | 28.23 | 1.04 | - | - |
| 2.4.2 | 2019 | VP [65] | 74.64 | 72.19 | -2.45 | 283.00 | 218.77 | 22.70 | 1.04 | 0.65 | 37.50 |
| PreResNet-29 | | | | | | | | | | | |
| 2.4.1 | 2019 | ED [72] | 75.70 | 65.11 | -10.59 | 41.28 | 3.91 | 90.52 | 0.27 | - | - |
| 2.4.1 | 2019 | ED [72] | 75.70 | 73.62 | -2.08 | 41.28 | 15.33 | 62.86 | 0.27 | - | - |
| PreResNet-101 | | | | | | | | | | | |
| 2.7.1 | 2020 | EB [64] | - | 72.29 | - | 7595 | 3038.00 | 60.00 | 44.54 | 13.36 | 70 |
| 2.7.1 | 2020 | EB [64] | - | 73.15 | - | 7595 | 5425.00 | 28.57 | 44.54 | 22.27 | 50 |
| 2.7.1 | 2020 | EB [64] | - | 73.52 | - | 7595 | 6329.17 | 16.67 | 44.54 | 31.18 | 30 |
| ResNeXt-20 | | | | | | | | | | | |
| 2.7.2 | 2020 | Hinge [66] | 71.95 | 71.26 | -0.69 | 36 | 19.29 | 46.41 | 0.21 | 0.14 | 34.76 |
| ResNeXt-164 | | | | | | | | | | | |
| 2.7.2 | 2020 | Hinge [66] | 76.87 | 77.44 | 0.57 | 210 | 100.28 | 52.25 | 1.70 | 0.99 | 41.51 |

TABLE 15: Other models on CIFAR-100, including DenseNet-40, PreResNet-29/101, and ResNeXt-20/164.

| Section | Year | Method | Baseline Top-1 Acc.(%) | Pruned Top-1 Acc.(%) | Top-1 Acc. ↓(%) | Baseline FLOPs (M) | Pruned FLOPs (M) | FLOPs ↓(%) | Baseline Params (M) | Pruned Params (M) | Params ↓(%) |
|---|---|---|---|---|---|---|---|---|---|---|---|
| AlexNet | | | | | | | | | | | |
| 2.3.3 | 2019 | OICSR [108] | 56.98 | 53.78 | -3.20 | 7270.00 | 2304.59 | 68.30 | 17.69 | - | - |
| 2.2.3 | 2018 | NISP [106] | - | - | 1.43 | 7270.00 | 2337.30 | 67.85 | 17.69 | 11.72 | 33.77 |
| 2.5.1 | 2018 | GDP-Lin [113] | 56.60 | 54.82 | -1.78 | 7270.00 | 2621.26 | 63.94 | 17.69 | - | - |
| 2.2.3 | 2018 | NISP [106] | - | - | 0.97 | 7270.00 | 2712.44 | 62.69 | 17.69 | 17.34 | 1.96 |
| 2.3.3 | 2019 | OICSR [108] | 56.98 | 56.83 | -0.15 | 7270.00 | 3344.20 | 54.00 | 17.69 | - | - |
| 2.2.3 | 2018 | NISP [106] | - | - | 0.54 | 7270.00 | 3366.01 | 53.70 | 17.69 | 17.18 | 2.91 |
| 2.5.1 | 2018 | GDP-Lin [113] | 56.60 | 55.83 | -0.77 | 7270.00 | 3469.12 | 52.28 | 17.69 | - | - |
| 2.2.2 | 2019 | AOFP [48] | 55.71 | 56.17 | 0.46 | 7270.00 | 4268.31 | 41.29 | 17.69 | - | - |
| 2.2.3 | 2018 | NISP [106] | - | - | 0.00 | 7270.00 | 4353.28 | 40.12 | 17.69 | 9.36 | 47.09 |
| 2.5.1 | 2018 | GDP-Lin [113] | 56.60 | 56.46 | -0.14 | 7270.00 | 4535.16 | 37.62 | 17.69 | - | - |
| 2.2.2 | 2019 | AOFP [48] | 55.71 | 56.54 | 0.83 | 7270.00 | 5014.39 | 31.03 | 17.69 | - | - |
| 2.3.3 | 2019 | OICSR [108] | 56.98 | 57.87 | 0.89 | 7270.00 | 5568.82 | 23.40 | 17.69 | - | - |

TABLE 16: AlexNet on ImageNet-1K.

| Section | Year | Method | Baseline Top-1 Acc.(%) | Pruned Top-1 Acc.(%) | Top-1 Acc. ↓(%) | Baseline FLOPs (M) | Pruned FLOPs (M) | FLOPs ↓(%) | Baseline Params (M) | Pruned Params (M) | Params ↓(%) |
|---|---|---|---|---|---|---|---|---|---|---|---|
| VGG-11 | | | | | | | | | | | |
| 2.1.2 | 2019 | COP [51] | 63.60 | 62.38 | -1.22 | 7630.00 | 4211.76 | 44.80 | 132.86 | 22.32 | 83.20 |
| 2.6.2 | 2021 | EE [61] | 70.84 | 71.15 | 0.31 | 7630.00 | 5035.80 | 34.00 | 132.86 | - | - |
| 2.4.1 | 2019 | Mol-19 [114] | 70.84 | 70.65 | -0.19 | 7630.00 | 6948.21 | 8.94 | 132.86 | 31.79 | 76.07 |
| VGG-16 | | | | | | | | | | | |
| 2.6.1 | 2022 | GNN-RL [85] | 70.50 | 70.99 | 0.49 | 15500 .00 | 3100.00 | 80.00 | 138.40 | - | - |
| 2.4.2 | 2019 | RBP [55] | - | 69.20 | - | 15500 .00 | 3100.00 | 80.00 | 138.40 | - | - |
| 2.6.1 | 2018 | AMC [103] | 70.50 | 69.10 | -1.40 | 15500 .00 | 3100.00 | 80.00 | 138.40 | - | - |
| 2.6.1 | 2021 | AGMC [86] | 70.50 | 70.35 | -0.15 | 15500 .00 | 3100.00 | 80.00 | 138.40 | - | - |
| 2.5.1 | 2018 | GDP-Lin [113] | 70.32 | 67.51 | -2.81 | 15500 .00 | 3800.00 | 75.48 | 138.40 | - | - |
| 2.6.2 | 2022 | DAIS [84] | - | - | 2.91 | 15500 .00 | 3875.00 | 75.00 | 138.40 | - | - |
| 2.2.2 | 2017 | ThiNet [115] | 68.34 | 67.34 | -1.00 | 15500 .00 | 4679.06 | 69.81 | 138.40 | 8.32 | 93.99 |
| 2.2.2 | 2017 | ThiNet [115] | 68.34 | 69.80 | 1.46 | 15500 .00 | 4799.29 | 69.04 | 138.40 | 131.50 | 4.99 |
| 2.5.1 | 2019 | DSG [116] | - | 71.44 | - | 15500 .00 | 5747.40 | 62.92 | 138.40 | - | - |
| 2.5.1 | 2018 | GDP-Lin [113] | 70.32 | 68.80 | -1.52 | 15500 .00 | 6400.00 | 58.71 | 138.40 | - | - |
| 2.7.2 | 2021 | CC [60] | 71.59 | 68.81 | -2.78 | 15500 .00 | 7379.52 | 52.39 | 138.40 | 8.37 | 93.95 |
| 2.5.1 | 2018 | GDP-Lin [113] | 70.32 | 69.88 | -0.44 | 15500 .00 | 7500.00 | 51.61 | 138.40 | - | - |
| 2.6.2 | 2022 | DAIS [84] | - | - | 1.64 | 15500 .00 | 7750.00 | 50.00 | 138.40 | - | - |
| 2.3.2 | 2018 | SSS [117] | - | 68.53 | - | 15500 .00 | - | - | 138.40 | - | - |
| 2.7.1 | 2022 | EarlyCroP [70] | - | 61.43 | - | 15500 .00 | - | - | 138.40 | 69.20 | 50.00 |
| 2.7.2 | 2020 | NM [118] | 73.36 | 61.18 | -12.18 | 15500 .00 | - | - | 138.40 | 85.25 | 38.41 |
| 2.7.2 | 2020 | NM [118] | 73.36 | 54.13 | -19.23 | 15500 .00 | - | - | 138.40 | 55.16 | 60.14 |
| 2.7.2 | 2020 | NM [118] | 73.36 | 43.99 | -29.37 | 15500 .00 | - | - | 138.40 | 64.19 | 53.62 |

TABLE 17: VGG-11/16 on ImageNet-1K.

| Section | Year | Method | Baseline Top-1 Acc.(%) | Pruned Top-1 Acc.(%) | Top-1 Acc. ↓(%) | Baseline FLOPs (M) | Pruned FLOPs (M) | FLOPs ↓(%) | Baseline Params (M) | Pruned Params (M) | Params ↓(%) |
|---|---|---|---|---|---|---|---|---|---|---|---|
| ResNet-18 | | | | | | | | | | | |
| 2.5.2 | 2021 | DDG [83] | 69.76 | 69.38 | -0.38 | 1814.00 | 758.25 | 58.20 | 11.69 | - | - |
| 2.5.2 | 2021 | ManiDP [81] | 69.76 | 68.35 | -1.41 | 1814.00 | 814.49 | 55.10 | 11.69 | - | - |
| 2.7.3 | 2022 | SOKS [54] | 70.42 | 69.16 | -1.26 | 1814.00 | 817.30 | 54.95 | 11.69 | 6.27 | 46.36 |
| 2.7.3 | 2020 | SWP [56] | 69.76 | 69.72 | -0.04 | 1814.00 | 823.92 | 54.58 | 11.69 | - | - |
| 2.2.1 | 2021 | LRMF [68] | 70.28 | 67.87 | -2.41 | 1814.00 | 847.14 | 53.30 | 11.69 | - | - |
| 2.6.2 | 2022 | MFP [91] | 70.28 | 67.11 | -3.17 | 1814.00 | 874.35 | 51.80 | 11.69 | - | - |
| 2.5.2 | 2022 | FTWT [53] | 69.76 | 67.49 | -2.27 | 1814.00 | 878.70 | 51.56 | 11.69 | - | - |
| 2.6.1 | 2022 | GNN-RL [85] | 69.76 | 68.66 | -1.10 | 1814.00 | 888.86 | 51.00 | 11.69 | - | - |
| 2.5.2 | 2021 | ManiDP [81] | 69.76 | 68.88 | -0.88 | 1814.00 | 888.86 | 51.00 | 11.69 | - | - |
| 2.7.3 | 2020 | SWP [56] | 69.76 | 69.98 | 0.22 | 1814.00 | 898.29 | 50.48 | 11.69 | - | - |
| 2.4.3 | 2022 | EKG [95] | 70.38 | 69.39 | -0.99 | 1814.00 | 905.19 | 50.10 | 11.69 | - | - |
| 2.5.2 | 2019 | FBS [119] | 70.71 | 68.17 | -2.54 | 1814.00 | 916.16 | 49.49 | 11.69 | - | - |
| 2.5.2 | 2021 | DDG [83] | 69.76 | 70.12 | 0.36 | 1814.00 | 917.88 | 49.40 | 11.69 | - | - |
| 2.5.2 | 2020 | DRLP [120] | 69.76 | 68.73 | -1.03 | 1814.00 | 935.05 | 48.45 | 11.69 | - | - |
| 2.6.3 | 2020 | ABCPruner [50] | 69.66 | 67.80 | -1.86 | 1814.00 | 962.55 | 46.94 | 11.69 | 9.50 | 18.73 |
| 2.6.2 | 2021 | EE [61] | 70.28 | 68.27 | -2.01 | 1814.00 | 968.68 | 46.60 | 11.69 | - | - |
| 2.3.2 | 2020 | SCOP [80] | 69.76 | 68.62 | -1.14 | 1814.00 | 997.70 | 45.00 | 11.69 | 6.60 | 43.50 |
| 2.6.3 | 2020 | ABCPruner [50] | 69.66 | 67.28 | -2.38 | 1814.00 | 999.91 | 44.88 | 11.69 | 6.60 | 43.54 |
| 2.3.2 | 2021 | ABP [39] | 70.29 | 67.83 | -2.46 | 1814.00 | 1021.28 | 43.70 | 11.69 | 6.31 | 46.00 |
| 2.6.2 | 2022 | DAIS [84] | 65.36 | 67.56 | 2.20 | 1814 | 1028.54 | 43.30 | 11.69 | - | - |
| 2.1.2 | 2019 | COP [51] | 70.29 | 66.98 | -3.31 | 1814.00 | 1028.54 | 43.30 | 11.69 | 6.42 | 45.10 |
| 2.2.3 | 2020 | PFP [37] | 69.74 | 65.65 | -4.09 | 1814.00 | 1031.80 | 43.12 | 11.69 | 4.62 | 60.48 |
| 2.6.2 | 2022 | DNCP [109] | 70.10 | 69.20 | -0.90 | 1814.00 | 1048.09 | 42.22 | 11.69 | - | - |
| 2.6.2 | 2020 | DMCP [121] | 70.10 | 68.40 | -1.90 | 1814.00 | 1048.09 | 42.22 | 11.69 | - | - |
| 2.6.2 | 2022 | MFP [91] | 70.28 | 67.66 | -2.62 | 1814.00 | 1055.75 | 41.80 | 11.69 | - | - |
| 2.5.1 | 2018 | SFP [90] | 70.28 | 67.10 | -3.18 | 1814.00 | 1055.75 | 41.80 | 11.69 | - | - |
| 2.1.2 | 2019 | FPGM [82] | 70.28 | 68.41 | -1.87 | 1814.00 | 1055.75 | 41.80 | 11.69 | - | - |
| 2.6.2 | 2022 | MFP [91] | 70.28 | 68.31 | -1.97 | 1814.00 | 1055.75 | 41.80 | 11.69 | - | - |
| 2.6.2 | 2020 | DSA [79] | 69.72 | 68.61 | -1.11 | 1814.00 | 1088.40 | 40.00 | 11.69 | - | - |
| 2.3.2 | 2020 | SCOP [80] | 69.76 | 69.18 | -0.58 | 1814.00 | 1110.17 | 38.80 | 11.69 | 7.10 | 39.30 |
| 2.6.2 | 2019 | TAS [88] | 67.65 | 69.15 | 1.50 | 1814.00 | 1209.94 | 33.30 | 11.69 | - | - |
| 2.2.3 | 2020 | PFP [37] | 69.74 | 67.38 | -2.36 | 1814.00 | 1282.50 | 29.30 | 11.69 | 6.57 | 43.80 |
| 2.4.1 | 2022 | SOSP [75] | 69.76 | 68.78 | -0.98 | 1814.00 | 1287.94 | 29.00 | 11.69 | 6.43 | 45.00 |
| 2.5.1 | 2021 | DCP-CAC [76] | 68.46 | 68.17 | -0.29 | 1814.00 | 1310.11 | 27.78 | 11.69 | 7.49 | 35.94 |
| 2.7.1 | 2020 | EB [64] | 69.57 | 68.28 | -1.29 | 1814.00 | 1372.19 | 24.36 | 11.69 | 8.18 | 30.00 |
| 2.4.1 | 2022 | SOSP [75] | 69.76 | 69.63 | -0.13 | 1814.00 | 1378.64 | 24.00 | 11.69 | 7.13 | 39.00 |
| 2.7.2 | 2020 | DJPQ [122] | 69.74 | 69.27 | -0.47 | 1814.00 | 1393.07 | 23.20 | 11.69 | - | - |
| 2.2.3 | 2020 | PFP [37] | 69.74 | 68.66 | -1.08 | 1814.00 | 1451.38 | 19.99 | 11.69 | 8.06 | 31.03 |
| 2.5.1 | 2021 | DCP-CAC [76] | 68.46 | 68.62 | 0.16 | 1814.00 | 1612.44 | 11.11 | 11.69 | 9.44 | 19.22 |
| 2.7.1 | 2020 | EB [64] | 69.57 | 69.84 | 0.27 | 1814.00 | 1695.89 | 6.51 | 11.69 | 10.52 | 10.00 |
| 2.5.1 | 2022 | CHEX [123] | - | 69.60 | - | 1814.00 | - | - | 11.69 | - | - |
| 2.6.3 | 2022 | EDropout [111] | 68.48 | 65.43 | -3.05 | 1814.00 | - | - | 11.69 | 5.39 | 53.91 |

TABLE 18: ResNet-18 on ImageNet-1K.

| Section | Year | Method | Baseline Top-1 Acc.(%) | Pruned Top-1 Acc.(%) | Top-1 Acc. ↓(%) | Baseline FLOPs (M) | Pruned FLOPs (M) | FLOPs ↓(%) | Baseline Params (M) | Pruned Params (M) | Params ↓(%) |
|---|---|---|---|---|---|---|---|---|---|---|---|
| ResNet-34 | | | | | | | | | | | |
| 2.5.2 | 2021 | DDG [83] | 73.31 | 71.95 | -1.36 | 3663 .00 | 1201.46 | 67.20 | 21.80 | - | - |
| 2.5.2 | 2021 | DDG [83] | 73.31 | 73.01 | -0.30 | 3663 .00 | 1490.84 | 59.30 | 21.80 | - | - |
| 2.6.3 | 2020 | ABCPruner [50] | 73.28 | 70.45 | -2.83 | 3663 .00 | 1503.10 | 58.97 | 21.80 | 10.47 | 51.96 |
| 2.7.3 | 2022 | SOKS [54] | 74.01 | 73.52 | -0.49 | 3663 .00 | 1612.52 | 55.98 | 21.80 | 11.27 | 48.30 |
| 2.5.2 | 2021 | ManiDP [81] | 73.31 | 72.74 | -0.57 | 3663 .00 | 1637.36 | 55.30 | 21.80 | - | - |
| 2.5.2 | 2022 | FTWT [53] | 73.30 | 71.71 | -1.59 | 3663 .00 | 1749.45 | 52.24 | 21.80 | - | - |
| 2.3.2 | 2021 | ABP [39] | 73.86 | 72.15 | -1.71 | 3663 .00 | 1923.08 | 47.50 | 21.80 | 10.75 | 50.70 |
| 2.5.2 | 2022 | FTWT [53] | 73.30 | 72.17 | -1.13 | 3663 .00 | 1926.01 | 47.42 | 21.80 | - | - |
| 2.5.2 | 2021 | ManiDP [81] | 73.31 | 73.30 | -0.01 | 3663 .00 | 1948.72 | 46.80 | 21.80 | - | - |
| 2.5.1 | 2022 | CHEX [123] | - | 73.50 | - | 3663 .00 | 1990.76 | 45.65 | 21.80 | - | - |
| 2.4.3 | 2022 | EKG [95] | 73.85 | 73.51 | -0.34 | 3663 .00 | 2010.99 | 45.10 | 21.80 | - | - |
| 2.3.2 | 2020 | SCOP [80] | 73.31 | 72.62 | -0.69 | 3663 .00 | 2021.98 | 44.80 | 21.80 | 11.86 | 45.60 |
| 2.6.2 | 2022 | DDNP [100] | 73.31 | 73.03 | -0.28 | 3663 .00 | 2043.95 | 44.20 | 21.80 | - | - |
| 2.2.3 | 2018 | NISP [106] | - | - | 0.92 | 3663 .00 | 2060.07 | 43.76 | 21.80 | 12.28 | 43.68 |
| 2.2.2 | 2020 | GFS [124] | 73.40 | 71.90 | -1.50 | 3663 .00 | 2060.44 | 43.75 | 21.80 | 14.70 | 32.57 |
| 2.3.2 | 2020 | DMC [102] | 73.30 | 72.57 | -0.73 | 3663 .00 | 2073.26 | 43.40 | 21.80 | - | - |
| 2.6.3 | 2022 | CCEP [59] | 73.30 | 72.67 | -0.63 | 3663 .00 | 2120.88 | 42.10 | 21.80 | - | - |
| 2.6.2 | 2022 | DAIS [84] | 72.23 | 72.77 | 0.54 | 3663 .00 | 2128.20 | 41.90 | 21.80 | - | - |
| 2.5.1 | 2018 | SFP [90] | 73.92 | 71.83 | -2.09 | 3663 .00 | 2157.51 | 41.10 | 21.80 | - | - |
| 2.1.2 | 2019 | FPGM [82] | 73.92 | 72.63 | -1.29 | 3663 .00 | 2157.51 | 41.10 | 21.80 | - | - |
| 2.6.3 | 2020 | ABCPruner [50] | 73.28 | 70.98 | -2.30 | 3663 .00 | 2161.19 | 41.00 | 21.80 | 10.07 | 53.79 |
| 2.3.2 | 2020 | SCOP [80] | 73.31 | 72.93 | -0.38 | 3663 .00 | 2230.77 | 39.10 | 21.80 | 13.15 | 39.70 |
| 2.5.2 | 2022 | FTWT [53] | 73.30 | 72.79 | -0.51 | 3663 .00 | 2279.48 | 37.77 | 21.80 | - | - |
| 2.2.2 | 2020 | GFS [124] | 73.40 | 73.50 | 0.10 | 3663 .00 | 2627.80 | 28.26 | 21.80 | 17.20 | 21.10 |
| 2.2.3 | 2018 | NISP [106] | - | - | 0.28 | 3663 .00 | 2662.27 | 27.32 | 21.80 | 15.88 | 27.14 |
| 2.5.2 | 2022 | FTWT [53] | 73.30 | 73.25 | -0.05 | 3663 .00 | 2715.75 | 25.86 | 21.80 | - | - |
| 2.6.3 | 2022 | CCEP [59] | 73.30 | 73.64 | 0.34 | 3663 .00 | 2731.13 | 25.44 | 21.80 | - | - |
| 2.3.3 | 2021 | GREG [97] | 73.31 | 73.61 | 0.30 | 3663 .00 | 2775.00 | 24.24 | 21.80 | - | - |
| 2.1.1 | 2017 | PFEC [69] | 73.23 | 72.17 | -1.06 | 3663 .00 | 2776.55 | 24.20 | 21.80 | 19.45 | 10.80 |
| 2.4.1 | 2019 | Mol-19 [114] | 73.31 | 72.83 | -0.48 | 3663 .00 | 2847.88 | 22.25 | 21.80 | 17.20 | 21.10 |
| 2.7.1 | 2022 | PaT [125] | - | 73.50 | - | 3663 .00 | 2897.55 | 20.90 | 21.80 | - | - |
| 2.1.1 | 2017 | PFEC [69] | 73.23 | 72.56 | -0.67 | 3663 .00 | 3099.46 | 15.38 | 21.80 | 20.08 | 7.87 |
| 2.6.3 | 2022 | EDropout [111] | 73.42 | 71.82 | -1.60 | 3663 .00 | - | - | 21.80 | 9.59 | 56.02 |
| 2.7.2 | 2020 | NM [118] | 73.31 | 66.77 | -6.54 | 3663 .00 | - | - | 21.80 | 19.72 | 9.52 |
| 2.7.2 | 2020 | NM [118] | 73.31 | 55.70 | -17.61 | 3663 .00 | - | - | 21.80 | 17.65 | 19.05 |
| 2.7.2 | 2020 | NM [118] | 73.31 | 37.43 | -35.88 | 3663 .00 | - | - | 21.80 | 15.57 | 28.57 |

TABLE 19: ResNet-34 on ImageNet-1K.

| Section | Year | Method | Baseline Top-1 Acc.(%) | Pruned Top-1 Acc.(%) | Top-1 Acc. ↓(%) | Baseline FLOPs (M) | Pruned FLOPs (M) | FLOPs ↓(%) | Baseline Params (M) | Pruned Params (M) | Params ↓(%) |
|---|---|---|---|---|---|---|---|---|---|---|---|
| ResNet-50 | | | | | | | | | | | |
| 2.6.2 | 2020 | DMCP [121] | 76.60 | 66.40 | -10.00 | 4089.00 | 277.25 | 93.22 | 25.56 | - | - |
| 2.7.3 | 2021 | JMDP [126] | 76.60 | 73.50 | -3.10 | 4089.00 | 897.59 | 78.05 | 25.56 | - | - |
| 2.5.1 | 2022 | SMCP [127] | 77.20 | 74.40 | -2.80 | 4089.00 | 897.59 | 78.05 | 25.56 | - | - |
| 2.1.2 | 2022 | CLR-RNF [49] | 76.01 | 71.11 | -4.90 | 4089.00 | 925.25 | 77.37 | 25.56 | 6.90 | 73.00 |
| 2.2.1 | 2021 | CHIP [42] | 76.15 | 73.30 | -2.85 | 4089.00 | 952.74 | 76.70 | 25.56 | 8.03 | 68.60 |
| 2.2.1 | 2020 | HRank [45] | 76.15 | 69.10 | -7.05 | 4089.00 | 979.76 | 76.04 | 25.56 | 8.29 | 67.57 |
| 2.5.1 | 2022 | SMCP [127] | 76.20 | 74.60 | -1.60 | 4089.00 | 997.32 | 75.61 | 25.56 | - | - |
| 2.5.1 | 2022 | CHEX [123] | - | 76.00 | - | 4089.00 | 997.32 | 75.61 | 25.56 | - | - |
| 2.3.1 | 2020 | EagleEye [101] | - | 74.20 | - | 4089.00 | 997.32 | 75.61 | 25.56 | - | - |
| 2.6.3 | 2019 | MetaPruning [128] | 76.60 | 73.40 | -3.20 | 4089.00 | 997.32 | 75.61 | 25.56 | - | - |
| 2.6.2 | 2022 | PaS [129] | 74.68 | 74.80 | 0.12 | 4089.00 | 997.32 | 75.61 | 25.56 | - | - |
| 2.4.1 | 2021 | GFP [130] | 76.79 | 73.94 | -2.85 | 4089.00 | 1020.00 | 75.06 | 25.56 | - | - |
| 2.6.2 | 2022 | DNCP [109] | 76.60 | 74.30 | -2.30 | 4089.00 | 1097.05 | 73.17 | 25.56 | - | - |
| 2.6.2 | 2020 | DMCP [121] | 76.60 | 74.40 | -2.20 | 4089.00 | 1097.05 | 73.17 | 25.56 | - | - |
| 2.3.2 | 2019 | GAL [63] | 76.15 | 69.31 | -6.84 | 4089.00 | 1109.73 | 72.86 | 25.56 | 10.22 | 60.00 |
| 2.2.2 | 2017 | ThiNet [115] | 72.88 | 68.42 | -4.46 | 4089.00 | 1165.26 | 71.50 | 25.56 | 8.68 | 66.04 |
| 2.6.1 | 2022 | DECORE [35] | 76.15 | 69.71 | -6.44 | 4089.00 | 1189.71 | 70.90 | 25.56 | 6.13 | 76.00 |
| 2.1.2 | 2022 | CLR-RNF [49] | 76.01 | 73.34 | -2.67 | 4089.00 | 1223.72 | 70.07 | 25.56 | 9.00 | 64.79 |
| 2.1.2 | 2022 | CLR-RNF [49] | 76.01 | 72.67 | -3.34 | 4089.00 | 1223.72 | 70.07 | 25.56 | 9.00 | 64.79 |
| 2.7.1 | 2020 | EB [64] | 75.99 | 70.16 | -5.83 | 4089.00 | 1282.37 | 68.64 | 25.56 | 7.67 | 70.00 |
| 2.5.2 | 2021 | DDG [83] | 76.13 | 75.12 | -1.01 | 4089.00 | 1312.57 | 67.90 | 25.56 | - | - |
| 2.3.3 | 2021 | GREG [97] | 76.13 | 73.90 | -2.23 | 4089.00 | 1336.27 | 67.32 | 25.56 | - | - |
| 2.4.1 | 2019 | Mol-19 [114] | 76.18 | 71.69 | -4.49 | 4089.00 | 1339.67 | 67.24 | 25.56 | 7.89 | 69.14 |
| 2.4.1 | 2022 | HAP [107] | 75.62 | 71.18 | -4.44 | 4089.00 | 1343.24 | 67.15 | 25.56 | 5.23 | 79.53 |
| 2.3.3 | 2021 | OTO [38] | 76.10 | 75.10 | -1.00 | 4089.00 | 1410.71 | 65.50 | 25.56 | 9.07 | 64.50 |
| 2.3.3 | 2021 | OTO [38] | 76.10 | 74.70 | -1.40 | 4089.00 | 1410.71 | 65.50 | 25.56 | 9.07 | 64.50 |
| 2.6.3 | 2022 | CCEP [59] | 76.13 | 74.87 | -1.26 | 4089.00 | 1468.36 | 64.09 | 25.56 | - | - |
| 2.3.2 | 2022 | WhiteBox [46] | 76.15 | 74.21 | -1.94 | 4089.00 | 1492.49 | 63.50 | 25.56 | - | - |
| 2.2.1 | 2021 | CHIP [42] | 76.15 | 75.26 | -0.89 | 4089.00 | 1521.11 | 62.80 | 25.56 | 11.07 | 56.70 |
| 2.7.2 | 2021 | CC [60] | 76.15 | 74.54 | -1.61 | 4089.00 | 1525.90 | 62.68 | 25.56 | 10.58 | 58.61 |
| 2.2.1 | 2020 | HRank [45] | 76.15 | 71.98 | -4.17 | 4089.00 | 1549.62 | 62.10 | 25.56 | 13.80 | 46.00 |
| 2.3.2 | 2021 | ResRep [93] | 76.15 | 75.30 | -0.85 | 4089.00 | 1549.73 | 62.10 | 25.56 | - | - |
| 2.3.2 | 2019 | GAL [63] | 76.15 | 69.88 | -6.27 | 4089.00 | 1579.61 | 61.37 | 25.56 | 14.70 | 42.47 |
| 2.3.3 | 2021 | GREG [97] | 76.13 | 74.93 | -1.20 | 4089.00 | 1597.27 | 60.94 | 25.56 | - | - |
| 2.6.1 | 2022 | DECORE [35] | 76.15 | 72.06 | -4.09 | 4089.00 | 1599.61 | 60.88 | 25.56 | 8.89 | 65.22 |
| 2.6.2 | 2020 | LFPC [92] | 76.15 | 74.46 | -1.69 | 4089.00 | 1602.89 | 60.80 | 25.56 | - | - |
| 2.6.2 | 2020 | LFPC [92] | 76.15 | 74.18 | -1.97 | 4089.00 | 1602.89 | 60.80 | 25.56 | - | - |
| 2.5.2 | 2021 | DDG [83] | 76.13 | 76.41 | 0.28 | 4089.00 | 1647.87 | 59.70 | 25.56 | - | - |
| 2.4.1 | 2022 | HAP [107] | 75.62 | 74.00 | -1.62 | 4089.00 | 1653.59 | 59.56 | 25.56 | 8.88 | 65.26 |
| 2.5.1 | 2018 | GDP-Lin [113] | 75.13 | 70.93 | -4.20 | 4089.00 | 1663.14 | 59.33 | 25.56 | - | - |
| 2.4.1 | 2022 | SOSP [75] | 76.15 | 73.38 | -2.77 | 4089.00 | 1676.49 | 59.00 | 25.56 | 9.97 | 61.00 |
| 2.7.1 | 2022 | PaT [125] | - | 74.85 | - | 4089.00 | 1690.45 | 58.66 | 25.56 | - | - |
| 2.2.2 | 2019 | AOFP [48] | 75.34 | 75.11 | -0.23 | 4089.00 | 1763.05 | 56.88 | 25.56 | - | - |
| 2.3.3 | 2021 | GREG [97] | 75.40 | 75.22 | -0.18 | 4089.00 | 1770.13 | 56.71 | 25.56 | - | - |
| 2.6.3 | 2020 | ABCPruner [50] | 76.01 | 73.52 | -2.49 | 4089.00 | 1774.19 | 56.61 | 25.56 | 11.24 | 56.03 |
| 2.6.3 | 2022 | CCEP [59] | 76.13 | 75.55 | -0.58 | 4089.00 | 1784.85 | 56.35 | 25.56 | - | - |
| 2.3.2 | 2021 | ResRep [93] | 76.15 | 75.97 | -0.18 | 4089.00 | 1794.66 | 56.11 | 25.56 | - | - |
| 2.6.2 | 2021 | EE [61] | 76.15 | 75.66 | -0.49 | 4089.00 | 1799.16 | 56.00 | 25.56 | - | - |
| 2.2.2 | 2017 | ThiNet [115] | 72.88 | 71.01 | -1.87 | 4089.00 | 1806.15 | 55.83 | 25.56 | 12.41 | 51.45 |
| 2.4.3 | 2019 | C-SGD [96] | 75.33 | 74.54 | -0.79 | 4089.00 | 1808.97 | 55.76 | 25.56 | - | - |
| 2.5.1 | 2021 | DCP-CAC [76] | - | - | -0.79 | 4089.00 | 1817.33 | 55.56 | 25.56 | 12.35 | 51.69 |
| 2.2.3 | 2018 | DCP [74] | - | - | 1.06 | 4089.00 | 1817.33 | 55.56 | 25.56 | 12.41 | 51.46 |
| 2.6.2 | 2022 | DAIS [84] | 72.75 | 74.45 | 1.70 | 4089.00 | 1827.78 | 55.30 | 25.56 | - | - |
| 2.1.2 | 2021 | SRR [87] | 76.13 | 75.11 | -1.02 | 4089.00 | 1835.96 | 55.10 | 25.56 | - | - |
| 2.3.1 | 2019 | GBN [94] | 74.51 | 75.18 | 0.67 | 4089.00 | 1837.60 | 55.06 | 25.56 | 11.91 | 53.40 |
| 2.3.2 | 2019 | GAL [63] | 76.15 | 71.80 | -4.35 | 4089.00 | 1839.55 | 55.01 | 25.56 | 19.36 | 24.27 |
| 2.3.2 | 2020 | DMC [102] | 76.15 | 75.35 | -0.80 | 4089.00 | 1840.05 | 55.00 | 25.56 | - | - |
| 2.4.3 | 2022 | EKG [95] | 77.00 | 76.60 | -0.40 | 4089.00 | 1840.05 | 55.00 | 25.56 | - | - |
| 2.6.1 | 2022 | RL-MCTS [41] | 77.34 | 76.46 | -0.88 | 4089.00 | 1840.05 | 55.00 | 25.56 | - | - |
| 2.6.2 | 2022 | DDNP [100] | 76.13 | 75.89 | -0.24 | 4089.00 | 1840.05 | 55.00 | 25.56 | - | - |
| 2.3.2 | 2020 | SCOP [80] | 76.15 | 75.26 | -0.89 | 4089.00 | 1856.41 | 54.60 | 25.56 | 12.32 | 51.80 |
| 2.4.2 | 2019 | RBP [55] | - | 73.00 | - | 4089.00 | 1858.64 | 54.55 | 25.56 | - | - |
| 2.3.2 | 2021 | ResRep [93] | 76.15 | 76.15 | 0.00 | 4089.00 | 1858.86 | 54.54 | 25.56 | - | - |
| 2.3.1 | 2020 | SCP [58] | 75.89 | 74.20 | 1.69 | 4089.00 | 1868.67 | 54.30 | 25.56 | - | - |
| 2.3.1 | 2020 | SCP [58] | 75.89 | 75.27 | 0.62 | 4089.00 | 1868.67 | 54.30 | 25.56 | - | - |
| 2.6.3 | 2020 | ABCPruner [50] | 76.01 | 73.86 | -2.15 | 4089.00 | 1869.25 | 54.29 | 25.56 | 11.75 | 54.03 |
| 2.4.1 | 2019 | CCP [99] | 76.15 | 76.98 | 0.83 | 4089.00 | 1876.85 | 54.10 | 25.56 | - | - |
| 2.3.1 | 2020 | PR [62] | 76.15 | 75.63 | 0.52 | 4089.00 | 1880.94 | 54.00 | 25.56 | - | - |
| 2.2.3 | 2022 | DLRFC [44] | 76.13 | 75.84 | 0.29 | 4089.00 | 1880.94 | 54.00 | 25.56 | 15.34 | 40.00 |
| 2.7.3 | 2021 | JMDP [126] | 76.60 | 76.00 | -0.60 | 4089.00 | 1894.90 | 53.66 | 25.56 | - | - |
| 2.5.1 | 2022 | SMCP [127] | 77.20 | 76.60 | -0.60 | 4089.00 | 1894.90 | 53.66 | 25.56 | - | - |

Continue on the next page...

TABLE 20: ResNet-50 on ImageNet-1K. (Part 1)

| Section | Year | Method | Baseline Top-1 Acc.(%) | Pruned Top-1 Acc.(%) | Top-1 Acc. ↓(%) | Baseline FLOPs (M) | Pruned FLOPs (M) | FLOPs ↓(%) | Baseline Params (M) | Pruned Params (M) | Params ↓(%) |
|---|---|---|---|---|---|---|---|---|---|---|---|
| ResNet-50 (cont.) | | | | | | | | | | | |
| 2.6.2 | 2022 | MFP [91] | 76.15 | 74.13 | -2.02 | 4089.00 | 1901.38 | 53.50 | 25.56 | - | - |
| 2.6.2 | 2022 | MFP [91] | 76.15 | 74.86 | -1.29 | 4089.00 | 1901.38 | 53.50 | 25.56 | - | - |
| 2.1.2 | 2019 | FPGM [82] | 76.15 | 75.59 | -0.56 | 4089.00 | 1901.38 | 53.50 | 25.56 | - | - |
| 2.7.2 | 2020 | Hinge [66] | - | 74.70 | - | 4089.00 | 1903.43 | 53.45 | 25.56 | - | - |
| 2.6.1 | 2022 | GNN-RL [85] | 76.10 | 74.28 | -1.82 | 4089.00 | 1921.83 | 53.00 | 25.56 | - | - |
| 2.7.2 | 2021 | CC [60] | 76.15 | 75.59 | -0.56 | 4089.00 | 1924.82 | 52.93 | 25.56 | 13.20 | 48.36 |
| 2.2.1 | 2021 | LRMF [68] | 76.15 | 74.70 | -1.45 | 4089.00 | 1934.10 | 52.70 | 25.56 | - | - |
| 2.5.1 | 2018 | GDP-Lin [113] | 75.13 | 71.89 | -3.24 | 4089.00 | 1991.53 | 51.30 | 25.56 | - | - |
| 2.5.1 | 2022 | SMCP [127] | 76.20 | 76.80 | 0.60 | 4089.00 | 1994.63 | 51.22 | 25.56 | - | - |
| 2.5.1 | 2022 | CHEX [123] | - | 77.40 | - | 4089.00 | 1994.63 | 51.22 | 25.56 | - | - |
| 2.3.1 | 2020 | EagleEye [101] | - | 76.40 | - | 4089.00 | 1994.63 | 51.22 | 25.56 | - | - |
| 2.6.3 | 2019 | MetaPruning [128] | 76.60 | 75.40 | -1.20 | 4089.00 | 1994.63 | 51.22 | 25.56 | - | - |
| 2.6.2 | 2022 | PaS [129] | 76.65 | 76.70 | 0.05 | 4089.00 | 1994.63 | 51.22 | 25.56 | - | - |
| 2.7.1 | 2022 | RRCP [105] | - | 75.13 | - | 4089.00 | 2003.20 | 51.01 | 25.56 | 13.83 | 45.88 |
| 2.4.1 | 2022 | SOSP [75] | 76.15 | 74.39 | -1.76 | 4089.00 | 2003.61 | 51.00 | 25.56 | 11.76 | 54.00 |
| 2.4.1 | 2021 | GFP [130] | 76.79 | 76.42 | -0.37 | 4089.00 | 2040.00 | 50.11 | 25.56 | - | - |
| 2.6.2 | 2020 | DSA [79] | 76.02 | 74.69 | -1.33 | 4089.00 | 2044.50 | 50.00 | 25.56 | - | - |
| 2.3.3 | 2019 | OICSR [108] | 76.31 | 75.95 | -0.36 | 4089.00 | 2044.50 | 50.00 | 25.56 | - | - |
| 2.4.1 | 2019 | CCP [99] | 76.15 | 76.80 | 0.65 | 4089.00 | 2093.57 | 48.80 | 25.56 | - | - |
| 2.2.1 | 2021 | CHIP [42] | 76.15 | 76.15 | 0.00 | 4089.00 | 2097.66 | 48.70 | 25.56 | 14.26 | 44.20 |
| 2.6.2 | 2022 | DNCP [109] | 76.60 | 76.30 | -0.30 | 4089.00 | 2194.10 | 46.34 | 25.56 | - | - |
| 2.6.2 | 2020 | DMCP [121] | 76.60 | 76.20 | -0.40 | 4089.00 | 2194.10 | 46.34 | 25.56 | - | - |
| 2.4.3 | 2019 | C-SGD [96] | 75.33 | 74.93 | -0.40 | 4089.00 | 2198.25 | 46.24 | 25.56 | - | - |
| 2.6.2 | 2021 | EE [61] | 76.15 | 76.05 | -0.10 | 4089.00 | 2203.97 | 46.10 | 25.56 | - | - |
| 2.6.1 | 2022 | RL-MCTS [41] | 77.34 | 76.80 | -0.54 | 4089.00 | 2203.97 | 46.10 | 25.56 | - | - |
| 2.3.2 | 2022 | WhiteBox [46] | 76.15 | 75.32 | -0.83 | 4089.00 | 2224.42 | 45.60 | 25.56 | - | - |
| 2.3.2 | 2020 | SCOP [80] | 76.15 | 75.95 | -0.20 | 4089.00 | 2236.68 | 45.30 | 25.56 | 14.62 | 42.80 |
| 2.4.1 | 2022 | SOSP [75] | 76.15 | 75.21 | -0.94 | 4089.00 | 2248.95 | 45.00 | 25.56 | 13.04 | 49.00 |
| 2.4.1 | 2019 | Mol-19 [114] | 76.18 | 74.50 | -1.68 | 4089.00 | 2249.45 | 44.99 | 25.56 | 14.18 | 44.53 |
| 2.2.1 | 2021 | CHIP [42] | 76.15 | 76.30 | 0.15 | 4089.00 | 2257.13 | 44.80 | 25.56 | 15.13 | 40.80 |
| 2.6.3 | 2022 | CCEP [59] | 76.13 | 76.06 | -0.07 | 4089.00 | 2266.94 | 44.56 | 25.56 | - | - |
| 2.4.1 | 2022 | HAP [107] | 75.62 | 75.36 | -0.26 | 4089.00 | 2268.99 | 44.51 | 25.56 | 13.74 | 46.26 |
| 2.3.3 | 2019 | OICSR [108] | 76.31 | 76.30 | -0.01 | 4089.00 | 2273.48 | 44.40 | 25.56 | - | - |
| 2.1.2 | 2021 | SRR [87] | 76.13 | 75.76 | -0.37 | 4089.00 | 2285.75 | 44.10 | 25.56 | - | - |
| 2.2.3 | 2018 | NISP [106] | - | - | 0.89 | 4089.00 | 2289.43 | 44.01 | 25.56 | 14.36 | 43.82 |
| 2.2.1 | 2020 | HRank [45] | 76.15 | 74.98 | -1.17 | 4089.00 | 2299.44 | 43.77 | 25.56 | 16.19 | 36.67 |
| 2.6.2 | 2019 | TAS [88] | 74.94 | 76.20 | 1.26 | 4089.00 | 2310.28 | 43.50 | 25.56 | - | - |
| 2.3.2 | 2019 | GAL [63] | 76.15 | 71.95 | -4.20 | 4089.00 | 2329.43 | 43.03 | 25.56 | 21.25 | 16.86 |
| 2.5.1 | 2021 | SEP [73] | 76.12 | 75.22 | -0.90 | 4089.00 | 2330.73 | 43.00 | 25.56 | - | - |
| 2.3.2 | 2021 | ABP [39] | 75.88 | 74.80 | -1.08 | 4089.00 | 2338.91 | 42.80 | 25.56 | 13.04 | 49.00 |
| 2.6.1 | 2022 | DECORE [35] | 76.15 | 74.58 | -1.57 | 4089.00 | 2359.42 | 42.30 | 25.56 | 14.13 | 44.71 |
| 2.6.2 | 2022 | MFP [91] | 76.15 | 75.67 | -0.48 | 4089.00 | 2363.44 | 42.20 | 25.56 | - | - |
| 2.5.1 | 2018 | GDP-Lin [113] | 75.13 | 72.61 | -2.52 | 4089.00 | 2372.89 | 41.97 | 25.56 | - | - |
| 2.5.1 | 2018 | SFP [90] | 76.15 | 62.14 | -14.01 | 4089.00 | 2379.80 | 41.80 | 25.56 | - | - |
| 2.5.1 | 2018 | SFP [90] | 76.15 | 74.61 | -1.54 | 4089.00 | 2379.80 | 41.80 | 25.56 | - | - |
| 2.3.1 | 2019 | GBN [94] | 76.50 | 76.19 | -0.31 | 4089.00 | 2431.32 | 40.54 | 25.56 | 17.42 | 31.83 |
| 2.1.2 | 2022 | CLR-RNF [49] | 76.01 | 74.85 | -1.16 | 4089.00 | 2437.48 | 40.39 | 25.56 | 16.92 | 33.80 |
| 2.6.2 | 2020 | DSA [79] | 76.02 | 75.10 | -0.92 | 4089.00 | 2453.40 | 40.00 | 25.56 | - | - |
| 2.7.1 | 2020 | EB [64] | 75.99 | 73.35 | -2.64 | 4089.00 | 2474.71 | 39.48 | 25.56 | 12.78 | 50.00 |
| 2.3.3 | 2019 | OICSR [108] | 76.31 | 76.53 | 0.22 | 4089.00 | 2563.80 | 37.30 | 25.56 | - | - |
| 2.2.2 | 2017 | ThiNet [115] | 72.88 | 72.04 | -0.84 | 4089.00 | 2584.76 | 36.79 | 25.56 | 16.98 | 33.57 |
| 2.4.3 | 2019 | C-SGD [96] | 75.33 | 75.27 | -0.06 | 4089.00 | 2586.29 | 36.75 | 25.56 | - | - |
| 2.4.1 | 2019 | Mol-19 [114] | 76.18 | 75.48 | -0.70 | 4089.00 | 2659.35 | 34.96 | 25.56 | 17.87 | 30.08 |
| 2.7.3 | 2022 | GKP-TMI [89] | 76.15 | 75.53 | -0.62 | 4089.00 | 2709.37 | 33.74 | 25.56 | 17.07 | 33.21 |
| 2.2.2 | 2019 | AOFP [48] | 75.34 | 75.63 | 0.29 | 4089.00 | 2740.16 | 32.99 | 25.56 | - | - |
| 2.3.3 | 2021 | GREG [97] | 76.13 | 76.13 | 0.00 | 4089.00 | 2744.30 | 32.89 | 25.56 | - | - |
| 2.7.3 | 2021 | JMDP [126] | 76.60 | 76.50 | -0.10 | 4089.00 | 2792.49 | 31.71 | 25.56 | - | - |
| 2.6.2 | 2020 | DMCP [121] | 76.60 | 77.00 | 0.40 | 4089.00 | 2792.49 | 31.71 | 25.56 | - | - |
| 2.2.3 | 2020 | PFP [37] | 76.13 | 75.21 | -0.92 | 4089.00 | 2860.26 | 30.05 | 25.56 | 14.30 | 44.04 |
| 2.4.1 | 2022 | SOSP [75] | 76.15 | 76.60 | 0.45 | 4089.00 | 2944.08 | 28.00 | 25.56 | 17.89 | 30.00 |
| 2.2.3 | 2018 | NISP [106] | - | - | 0.21 | 4089.00 | 2972.29 | 27.31 | 25.56 | 18.63 | 27.12 |
| 2.4.1 | 2022 | SOSP [75] | 76.15 | 75.85 | -0.30 | 4089.00 | 2984.97 | 27.00 | 25.56 | 15.34 | 40.00 |
| 2.6.3 | 2019 | MetaPruning [128] | 76.60 | 76.20 | -0.40 | 4089.00 | 2991.95 | 26.83 | 25.56 | - | - |
| 2.6.2 | 2022 | PaS [129] | 77.53 | 77.60 | 0.07 | 4089.00 | 2991.95 | 26.83 | 25.56 | - | - |
| 2.5.1 | 2022 | SMCP [127] | 76.20 | 77.10 | 0.90 | 4089.00 | 2991.95 | 26.83 | 25.56 | - | - |
| 2.3.1 | 2020 | EagleEye [101] | - | 77.10 | - | 4089.00 | 2991.95 | 26.83 | 25.56 | - | - |
| 2.4.1 | 2021 | GFP [130] | 76.79 | 76.95 | 0.16 | 4089.00 | 3060.00 | 25.17 | 25.56 | - | - |
| 2.5.1 | 2022 | SMCP [127] | 77.20 | 77.60 | 0.40 | 4089.00 | 3091.68 | 24.39 | 25.56 | - | - |
| 2.7.3 | 2022 | GKP-TMI [89] | 76.15 | 75.96 | -0.19 | 4089.00 | 3168.98 | 22.50 | 25.56 | 19.91 | 22.10 |
| 2.7.1 | 2020 | EB [64] | 75.99 | 73.86 | -2.13 | 4089.00 | 3228.48 | 21.04 | 25.56 | 17.89 | 30.00 |
| 2.4.1 | 2022 | SOSP [75] | 76.15 | 76.56 | 0.41 | 4089.00 | 3230.31 | 21.00 | 25.56 | 19.94 | 22.00 |
| 2.4.1 | 2019 | Mol-19 [114] | 76.18 | 76.43 | 0.25 | 4089.00 | 3269.20 | 20.05 | 25.56 | 22.56 | 11.72 |
| 2.6.1 | 2022 | DECORE [35] | 76.15 | 76.31 | 0.16 | 4089.00 | 3539.13 | 13.45 | 25.56 | 22.74 | 11.02 |
| 2.2.3 | 2020 | PFP [37] | 76.13 | 75.91 | -0.22 | 4089.00 | 3646.57 | 10.82 | 25.56 | 20.96 | 18.01 |
| 2.6.3 | 2022 | EDropout [111] | 75.27 | 73.72 | -1.55 | 4089.00 | - | - | 25.56 | 10.86 | 57.50 |
| 2.7.3 | 2022 | 1xN [131] | 77.01 | 76.65 | -0.35 | 4089.00 | - | - | 25.56 | 12.78 | 50.00 |

TABLE 20: ResNet-50 on ImageNet-1K. (Part 2)

| Section | Year | Method | Baseline Top-1 Acc.(%) | Pruned Top-1 Acc.(%) | Top-1 Acc. ↓(%) | Baseline FLOPs (M) | Pruned FLOPs (M) | FLOPs ↓(%) | Baseline Params (M) | Pruned Params (M) | Params ↓(%) |
|---|---|---|---|---|---|---|---|---|---|---|---|
| ResNet-101 | | | | | | | | | | | |
| 2.4.1 | 2019 | MoI-19 [114] | 77.37 | 74.16 | -3.21 | 7801.00 | 1760.23 | 77.44 | 44.55 | 13.55 | 69.57 |
| 2.5.1 | 2022 | CHEX [123] | - | 77.60 | - | 7801.00 | 1957.98 | 74.90 | 44.55 | - | - |
| 2.6.3 | 2020 | ABCPruner [50] | 77.38 | 74.76 | -2.62 | 7801.00 | 1958.69 | 74.89 | 44.55 | 12.94 | 70.95 |
| 2.5.1 | 2022 | SMCP [127] | 77.40 | 76.80 | -0.60 | 7801.00 | 2000.26 | 74.36 | 44.55 | - | - |
| 2.4.1 | 2019 | MoI-19 [114] | 77.37 | 75.38 | -1.99 | 7801.00 | 2470.32 | 68.33 | 44.55 | 17.74 | 60.18 |
| 2.5.1 | 2022 | SMCP [127] | 77.40 | 77.30 | -0.10 | 7801.00 | 2600.33 | 66.67 | 44.55 | - | - |
| 2.4.1 | 2019 | MoI-19 [114] | 77.37 | 75.27 | -2.10 | 7801.00 | 2850.37 | 63.46 | 44.55 | 20.63 | 53.69 |
| 2.3.2 | 2020 | SCOP [80] | 77.37 | 77.36 | -0.01 | 7801.00 | 3104.80 | 60.20 | 44.55 | 18.80 | 57.80 |
| 2.6.3 | 2020 | ABCPruner [50] | 77.38 | 75.82 | -1.56 | 7801.00 | 3137.80 | 59.78 | 44.55 | 17.72 | 60.22 |
| 2.3.2 | 2020 | DMC [102] | 77.37 | 77.40 | 0.03 | 7801.00 | 3432.44 | 56.00 | 44.55 | - | - |
| 2.5.1 | 2022 | CHEX [123] | - | 78.80 | - | 7801.00 | 3503.75 | 55.09 | 44.55 | - | - |
| 2.5.1 | 2022 | SMCP [127] | 77.40 | 77.80 | 0.40 | 7801.00 | 3600.46 | 53.85 | 44.55 | - | - |
| 2.3.1 | 2018 | RSNLI [132] | 76.40 | 74.56 | -1.84 | 7801.00 | 3690.47 | 52.69 | 44.55 | 17.37 | 61.00 |
| 2.2.2 | 2019 | AOFP [48] | 76.63 | 76.40 | -0.23 | 7801.00 | 3885.04 | 50.20 | 44.55 | - | - |
| 2.4.1 | 2021 | GFP [130] | 78.29 | 78.33 | 0.04 | 7801.00 | 3900.00 | 50.01 | 44.55 | - | - |
| 2.3.1 | 2018 | RSNLI [132] | 76.40 | 75.27 | -1.13 | 7801.00 | 3962.55 | 49.20 | 44.55 | 23.61 | 47.00 |
| 2.5.1 | 2022 | SMCP [127] | 77.40 | 78.10 | 0.70 | 7801.00 | 4000.51 | 48.72 | 44.55 | - | - |
| 2.3.2 | 2020 | SCOP [80] | 77.37 | 77.75 | 0.38 | 7801.00 | 4009.71 | 48.60 | 44.55 | 23.70 | 46.80 |
| 2.1.2 | 2019 | FPGM [82] | 77.37 | 77.32 | -0.05 | 7801.00 | 4134.53 | 47.00 | 44.55 | - | - |
| 2.2.3 | 2020 | PFP [37] | 77.37 | 76.43 | -0.94 | 7801.00 | 4284.31 | 45.08 | 44.55 | 22.07 | 50.45 |
| 2.5.1 | 2018 | SFP [90] | 77.37 | 77.51 | 0.14 | 7801.00 | 4508.98 | 42.20 | 44.55 | - | - |
| 2.5.1 | 2018 | SFP [90] | 77.37 | 77.03 | -0.34 | 7801.00 | 4508.98 | 42.20 | 44.55 | - | - |
| 2.4.1 | 2019 | MoI-19 [114] | 77.37 | 77.35 | -0.02 | 7801.00 | 4700.60 | 39.74 | 44.55 | 31.10 | 30.20 |
| 2.2.2 | 2019 | AOFP [48] | 76.63 | 76.88 | 0.25 | 7801.00 | 5451.43 | 30.12 | 44.55 | - | - |
| 2.2.3 | 2020 | PFP [37] | 77.37 | 76.78 | -0.59 | 7801.00 | 5509.07 | 29.38 | 44.55 | 29.83 | 33.04 |
| 2.6.3 | 2022 | EDropout [111] | 75.94 | 73.94 | -2.00 | 7801.00 | - | - | 44.55 | 19.13 | 57.07 |
| ResNet-152 | | | | | | | | | | | |
| 2.6.3 | 2020 | ABCPruner [50] | 78.31 | 76.00 | -2.31 | 11514.00 | 2697.93 | 76.57 | 60.19 | 15.62 | 74.05 |
| 2.2.2 | 2019 | AOFP [48] | 77.37 | 76.40 | -0.97 | 11514.00 | 2858.09 | 75.18 | 60.19 | - | - |
| 2.2.2 | 2019 | AOFP [48] | 77.37 | 77.00 | -0.37 | 11514.00 | 4215.68 | 63.39 | 60.19 | - | - |
| 2.6.3 | 2020 | ABCPruner [50] | 78.31 | 77.12 | -1.19 | 11514.00 | 4275.39 | 62.87 | 60.19 | 24.07 | 60.01 |
| 2.2.2 | 2019 | AOFP [48] | 77.37 | 77.47 | 0.10 | 11514.00 | 6246.96 | 45.74 | 60.19 | - | - |

TABLE 21: ResNet-101/152 on ImageNet-1K.

| Section | Year | Method | Baseline Top-1 Acc.(%) | Pruned Top-1 Acc.(%) | Top-1 Acc. ↓(%) | Baseline FLOPs (M) | Pruned FLOPs (M) | FLOPs ↓(%) | Baseline Params (M) | Pruned Params (M) | Params ↓(%) |
|---|---|---|---|---|---|---|---|---|---|---|---|
| MobileNet-V1 | | | | | | | | | | | |
| 2.6.3 | 2019 | MetaPruning [128] | 70.60 | 57.20 | -13.40 | 569.00 | 41.00 | 92.79 | 4.20 | - | - |
| 2.6.3 | 2019 | MetaPruning [128] | 70.60 | 66.10 | -4.50 | 569.00 | 149.00 | 73.81 | 4.20 | - | - |
| 2.5.1 | 2022 | SMCP [127] | 72.60 | 68.30 | -4.30 | 569.00 | 208.00 | 63.44 | 4.20 | - | - |
| 2.6.1 | 2018 | AMC [103] | 70.60 | 68.90 | -1.70 | 569.00 | 227.60 | 60.00 | 4.20 | - | - |
| 2.6.1 | 2021 | AGMC [86] | 70.60 | 69.40 | -1.20 | 569.00 | 227.60 | 60.00 | 4.20 | - | - |
| 2.6.1 | 2022 | GNN-RL [85] | 70.90 | 69.50 | -1.40 | 569.00 | 227.60 | 60.00 | 4.20 | - | - |
| 2.3.1 | 2020 | EagleEye [101] | - | 70.90 | - | 569.00 | 284.00 | 50.09 | 4.20 | - | - |
| 2.4.3 | 2022 | RollBack [104] | - | 49.34 | - | 569.00 | 284.50 | 50.00 | 4.20 | - | - |
| 2.5.2 | 2020 | DRLP [120] | 70.90 | 70.60 | -0.30 | 569.00 | 284.50 | 50.00 | 4.20 | - | - |
| 2.6.1 | 2018 | AMC [103] | 70.60 | 70.20 | -0.40 | 569.00 | 284.50 | 50.00 | 4.20 | - | - |
| 2.6.3 | 2019 | MetaPruning [128] | 70.60 | 70.90 | 0.30 | 569.00 | 324.00 | 43.06 | 4.20 | - | - |
| 2.5.2 | 2022 | FTWT [53] | 69.57 | 69.66 | 0.09 | 569.00 | 335.31 | 41.07 | 4.20 | - | - |
| 2.5.1 | 2022 | SMCP [127] | 72.60 | 71.00 | -1.60 | 569.00 | 356.00 | 37.43 | 4.20 | - | - |
| 2.7.3 | 2022 | 1xN [131] | 71.15 | 70.28 | -0.87 | 569.00 | - | - | 4.20 | 2.10 | 50 |
| MobileNet-V2 | | | | | | | | | | | |
| 2.6.3 | 2019 | MetaPruning [128] | 74.70 | 58.30 | -16.40 | 300.00 | 22.05 | 92.65 | 3.50 | - | - |
| 2.6.2 | 2020 | DMCP [121] | 72.30 | 59.10 | -13.30 | 300.00 | 43.00 | 85.67 | 3.50 | - | - |
| 2.6.3 | 2019 | MetaPruning [128] | 74.70 | 63.80 | -10.90 | 300.00 | 43.08 | 85.64 | 3.50 | - | - |
| 2.6.3 | 2019 | MetaPruning [128] | 74.70 | 65.00 | -9.70 | 300.00 | 53.85 | 82.05 | 3.50 | - | - |
| 2.6.2 | 2020 | DMCP [121] | 72.30 | 62.70 | -9.70 | 300.00 | 59.00 | 80.33 | 3.50 | - | - |
| 2.6.3 | 2019 | MetaPruning [128] | 74.70 | 67.30 | -7.40 | 300.00 | 63.59 | 78.80 | 3.50 | - | - |
| 2.6.3 | 2019 | MetaPruning [128] | 74.70 | 68.20 | -6.50 | 300.00 | 71.79 | 76.07 | 3.50 | - | - |
| 2.6.2 | 2020 | DMCP [121] | 72.30 | 66.10 | -6.30 | 300.00 | 87.00 | 71.00 | 3.50 | - | - |
| 2.4.1 | 2021 | GFP [130] | 75.74 | 65.94 | -9.80 | 300.00 | 90.00 | 70.00 | 3.50 | - | - |
| 2.6.2 | 2022 | DNCP [109] | 72.30 | 66.50 | -5.80 | 300.00 | 97.00 | 67.67 | 3.50 | - | - |
| 2.6.2 | 2020 | DMCP [121] | 72.30 | 67.00 | -5.30 | 300.00 | 97.00 | 67.67 | 3.50 | - | - |
| 2.2.2 | 2020 | GFS [124] | 72.00 | 66.90 | -5.10 | 300.00 | 102.23 | 65.92 | 3.50 | 1.90 | 45.71 |
| 2.2.2 | 2020 | GFS [124] | 72.00 | 68.80 | -3.20 | 300.00 | 131.85 | 56.05 | 3.50 | 2.00 | 42.86 |
| 2.2.2 | 2020 | GFS [124] | 72.00 | 69.70 | -2.30 | 300.00 | 145.22 | 51.59 | 3.50 | 2.20 | 37.14 |
| 2.5.2 | 2021 | ManiDP [81] | 71.80 | 69.62 | -2.18 | 300.00 | 146.40 | 51.20 | 3.50 | - | - |
| 2.6.3 | 2019 | MetaPruning [128] | 74.70 | 72.70 | -2.00 | 300.00 | 149.23 | 50.26 | 3.50 | - | - |
| 2.4.1 | 2021 | GFP [130] | 75.74 | 69.16 | -6.58 | 300.00 | 150.00 | 50.00 | 3.50 | - | - |
| 2.3.2 | 2020 | DMC [102] | 71.88 | 68.37 | -3.51 | 300.00 | 162.00 | 46.00 | 3.50 | - | - |
| 2.2.2 | 2020 | GFS [124] | 72.00 | 70.40 | -1.60 | 300.00 | 162.42 | 45.86 | 3.50 | 2.30 | 34.29 |
| 2.5.2 | 2021 | DDG [83] | 71.88 | 71.62 | -0.26 | 300.00 | 168.00 | 44.00 | 3.50 | - | - |
| 2.6.1 | 2022 | GNN-RL [85] | 71.87 | 70.04 | -1.83 | 300.00 | 174.00 | 42.00 | 3.50 | - | - |
| 2.4.2 | 2019 | RBP [55] | - | 69.70 | - | 300.00 | 176.47 | 41.18 | 3.50 | - | - |
| 2.4.3 | 2022 | RollBack [104] | - | 52.86 | - | 300.00 | 180.00 | 40.00 | 3.50 | - | - |
| 2.5.2 | 2021 | ManiDP [81] | 71.80 | 71.42 | -0.38 | 300.00 | 188.40 | 37.20 | 3.50 | - | - |
| 2.2.2 | 2020 | GFS [124] | 72.00 | 71.20 | -0.80 | 300.00 | 192.04 | 35.99 | 3.50 | 2.70 | 22.86 |
| 2.6.1 | 2021 | AGMC [86] | 71.80 | 70.87 | -0.93 | 300.00 | 210.00 | 30.00 | 3.50 | - | - |
| 2.2.3 | 2022 | DLRFC [44] | 71.80 | 71.88 | -0.08 | 300.00 | 210.0 | 30.00 | - | - | - |
| 2.6.1 | 2018 | AMC [103] | 71.80 | 70.80 | -1.00 | 300.00 | 210.00 | 30.00 | 3.50 | - | - |
| 2.2.2 | 2020 | GFS [124] | 72.00 | 71.60 | -0.40 | 300.00 | 210.19 | 29.94 | 3.50 | 2.90 | 17.14 |
| 2.6.2 | 2022 | DNCP [109] | 72.30 | 72.70 | 0.40 | 300.00 | 211.00 | 29.67 | 3.50 | - | - |
| 2.6.2 | 2020 | DMCP [121] | 72.30 | 73.50 | 1.20 | 300.00 | 211.00 | 29.67 | 3.50 | - | - |
| 2.6.2 | 2020 | DMCP [121] | 72.30 | 72.40 | 0.10 | 300.00 | 211.00 | 29.67 | 3.50 | - | - |
| 2.6.2 | 2022 | DDNP [100] | 72.05 | 72.20 | 0.15 | 300.00 | 211.50 | 29.50 | 3.50 | - | - |
| 2.7.1 | 2022 | RRCP [105] | - | 70.90 | - | 300.00 | 212.61 | 29.13 | 3.50 | - | - |
| 2.7.2 | 2021 | CC [60] | 71.88 | 70.91 | -0.97 | 300.00 | 215.00 | 28.33 | 3.50 | - | - |
| 2.3.1 | 2020 | PR [62] | 72.00 | 71.80 | 0.20 | 300.00 | 216.00 | 28.00 | 3.50 | - | - |
| 2.2.2 | 2020 | GFS [124] | 72.00 | 71.90 | -0.10 | 300.00 | 246.50 | 17.83 | 3.50 | 3.20 | 8.57 |
| 2.6.2 | 2020 | DMCP [121] | 72.30 | 73.90 | 1.60 | 300.00 | 300.00 | 0.00 | 3.50 | - | - |
| 2.6.2 | 2020 | DMCP [121] | 72.30 | 74.60 | 2.30 | 300.00 | 300.00 | 0.00 | 3.50 | - | - |
| 2.7.3 | 2022 | 1xN [131] | 71.74 | 70.23 | -1.50 | 300.00 | - | - | 3.50 | 1.75 | 50 |
| MobileNet-V3-Small | | | | | | | | | | | |
| 2.2.2 | 2020 | GFS [124] | 67.50 | 65.80 | -1.70 | - | - | 23.44 | - | - | 20.00 |

TABLE 22: MobileNet-V1/V2/V3-Small on ImageNet-1K.

| Section | Year | Method | Baseline Top-1 Acc.(%) | Pruned Top-1 Acc.(%) | Top-1 Acc. ↓(%) | Baseline FLOPs (M) | Pruned FLOPs (M) | FLOPs ↓(%) | Baseline Params (M) | Pruned Params (M) | Params ↓(%) |
|---|---|---|---|---|---|---|---|---|---|---|---|
| ProxylessNet-Mobile | | | | | | | | | | | |
| 2.2.2 | 2020 | GFS [124] | 74.60 | 74.00 | -0.60 | 324.00 | 232.00 | 28.40 | 4.10 | 3.40 | 17.07 |
| GoogLeNet | | | | | | | | | | | |
| 2.2.3 | 2018 | NISP [106] | - | - | 0.21 | 1560.00 | 649.90 | 58.34 | 6.80 | 4.50 | 33.76 |
| ResNeXt-50 | | | | | | | | | | | |
| 2.4.1 | 2021 | GFP [130] | 77.97 | 77.53 | -0.44 | 4230.00 | 2110.00 | 50.12 | 25.02 | - | - |
| NAS | | | | | | | | | | | |
| 2.7.2 | 2021 | NPAS [133] | - | 68.30 | - | - | 98.00 | - | - | 2.80 | - |
| 2.7.1 | 2022 | SuperTickets [134] | - | 74.20 | - | - | 125 | - | - | 2.70 | - |
| 2.7.2 | 2021 | NPAS [133] | - | 70.90 | - | - | 147.00 | - | - | 3.00 | - |
| 2.7.2 | 2021 | NPAS [133] | - | 75.00 | - | - | 201.00 | - | - | 3.50 | - |
| 2.7.2 | 2021 | NPAS [133] | - | 78.20 | - | - | 385.00 | - | - | 5.30 | - |
| 2.6.2 | 2022 | ReCNAS [112] | - | 76.90 | - | - | - | - | - | 6.30 | - |
| 2.6.2 | 2022 | ReCNAS [112] | - | 75.20 | - | - | - | - | - | 5.20 | - |
| 2.6.2 | 2022 | ReCNAS [112] | - | 77.10 | - | - | - | - | - | 6.80 | - |

TABLE 23: Other models on ImageNet-1K, including ProxylessNet-Mobile, GoogLeNet, ResNeXt-50, and models searched by Neural Architecture Search (NAS).

# References


[1] Y. LeCun, J. Denker, and S. Solla, "Optimal brain damage," in *Proc. Adv. Neural Inform. Process. Syst.*, 1989, p. 598–605.

[2] S. Han, J. Pool, J. Tran, and W. Dally, "Learning both weights and connections for efficient neural network," in *Proc. Adv. Neural Inform. Process. Syst.*, 2015, p. 1135–1143.

[3] Y. Guo, A. Yao, and Y. Chen, "Dynamic network surgery for efficient dnns," in *Proc. Adv. Neural Inform. Process. Syst.*, 2016, p. 1387–1395.

[4] S. Han, H. Mao, and W. J. Dally, "Deep compression: Compressing deep neural networks with pruning, trained quantization and huffman coding," in *Proc. Int. Conf. Learn. Represent.*, 2016.

[5] K. Simonyan and A. Zisserman, "Very deep convolutional networks for large-scale image recognition," in *Proc. Int. Conf. Learn. Represent.*, 2015.

[6] M. Rastegari, V. Ordonez, J. Redmon, and A. Farhadi, "Xnor-net: Imagenet classification using binary convolutional neural networks," in *Proc. Eur. Conf. Comput. Vis.* Springer, 2016, pp. 525–542.

[7] I. Hubara, M. Courbariaux, D. Soudry, R. El-Yaniv, and Y. Bengio, "Binarized neural networks," in *Proc. Adv. Neural Inform. Process. Syst.*, 2016, p. 4114–4122.

[8] J. Ott, Z. Lin, Y. Zhang, S.-C. Liu, and Y. Bengio, "Recurrent neural networks with limited numerical precision," *arXiv preprint arXiv:1608.06902*, 2016.

[9] C. Zhu, S. Han, H. Mao, and W. J. Dally, "Trained ternary quantization," in *Proc. Int. Conf. Learn. Represent.*, 2017.

[10] T. Liang, J. Glossner, L. Wang, S. Shi, and X. Zhang, "Pruning and quantization for deep neural network acceleration: A survey," *Neurocomputing*, vol. 461, pp. 370–403, 2021.

[11] F. Tung and G. Mori, "Clip-q: Deep network compression learning by in-parallel pruning-quantization," in *Proc. IEEE Conf. Comput. Vis. Pattern Recog.*, 2018.

[12] S. J. Kwon, D. Lee, B. Kim, P. Kapoor, B. Park, and G.-Y. Wei, "Structured compression by weight encryption for unstructured pruning and quantization," in *Proc. IEEE Conf. Comput. Vis. Pattern Recog.*, 2020, pp. 1909–1918.

[13] T. N. Sainath, B. Kingsbury, V. Sindhwani, E. Arisoy, and B. Ramabhadran, "Low-rank matrix factorization for deep neural network training with high-dimensional output targets," in *2013 Proc. IEEE Int. Conf. Acoust. Speech Signal Process.* IEEE, 2013, pp. 6655–6659.

[14] J. Xue, J. Li, D. Yu, M. Seltzer, and Y. Gong, "Singular value decomposition based low-footprint speaker adaptation and personalization for deep neural network," in *2014 Proc. IEEE Int. Conf. Acoust. Speech Signal Process.* IEEE, 2014, pp. 6359–6363.

[15] I. Aizenberg, A. Luchetta, and S. Manetti, "A modified learning algorithm for the multilayer neural network with multi-valued neurons based on the complex qr decomposition," *Soft Comput.*, vol. 16, no. 4, pp. 563–575, 2012.

[16] Y.-D. Kim, E. Park, S. Yoo, T. Choi, L. Yang, and D. Shin, "Compression of deep convolutional neural networks for fast and low power mobile applications," in *Proc. Int. Conf. Learn. Represent.*, 2015.

[17] M. Janzamin, H. Sedghi, and A. Anandkumar, "Beating the perils of non-convexity: Guaranteed training of neural networks using tensor methods," *arXiv preprint arXiv:1506.08473*, 2015.

[18] A. Cichocki, D. Mandic, L. De Lathauwer, G. Zhou, Q. Zhao, C. Caiafa, and H. A. Phan, "Tensor decompositions for signal processing applications: From two-way to multiway component analysis," *IEEE Signal Process. Mag.*, vol. 32, no. 2, pp. 145–163, 2015.

[19] L. Liebenwein, A. Maalouf, D. Feldman, and D. Rus, "Compressing neural networks: Towards determining the optimal layer-wise decomposition," in *Proc. Adv. Neural Inform. Process. Syst.*, vol. 34, 2021, pp. 5328–5344.

[20] M. G. A. Hameed, M. S. Tahaei, A. Mosleh, and V. P. Nia, "Convolutional neural network compression through generalized kronecker product decomposition," in *Proc. AAAI Conf. Artif. Intell.*, vol. 36, no. 1, 2022, pp. 771–779.

[21] M. Lin, L. Cao, S. Li, Q. Ye, Y. Tian, J. Liu, Q. Tian, and R. Ji, "Filter sketch for network pruning," *IEEE Trans. Neural Netw. Learn Syst.*, vol. 33, no. 12, pp. 7091–7100, 2022.

[22] C. Buciluǎ, R. Caruana, and A. Niculescu-Mizil, "Model compression," in *Proc. 12th ACM SIGKDD Int. Conf. Knowl. Discov. Data Min.*, 2006, pp. 535–541.

[23] G. Hinton, O. Vinyals, and J. Dean, "Distilling the knowledge in a neural network," in *NeurIPS Deep Learn. Represent. Learn. Workshop*, 2015.

[24] R. Anil, G. Pereyra, A. Passos, R. Ormandi, G. E. Dahl, and G. E. Hinton, "Large scale distributed neural network training through online distillation," in *Proc. Int. Conf. Learn. Represent.*, 2018.

[25] L. Zhang, J. Song, A. Gao, J. Chen, C. Bao, and K. Ma, "Be your own teacher: Improve the performance of convolutional neural networks via self distillation," in *Proc. Int. Conf. Comput. Vis.*, 2019, pp. 3713–3722.

[26] T. Li, J. Li, Z. Liu, and C. Zhang, "Few sample knowledge distillation for efficient network compression," in *Proc. IEEE Conf. Comput. Vis. Pattern Recog.*, 2020, pp. 14 639–14 647.

[27] H. Bai, J. Wu, I. King, and M. Lyu, "Few shot network compression via cross distillation," in *Proc. AAAI Conf. Artif. Intell.*, vol. 34, no. 04, 2020, pp. 3203–3210.

[28] H. Wang, J. Liu, X. Ma, Y. Yong, Z. Chai, and J. Wu, "Compressing models with few samples: Mimicking then replacing," in *Proc. IEEE Conf. Comput. Vis. Pattern Recog.*, 2022, pp. 701–710.

[29] T. Elsken, J. H. Metzen, and F. Hutter, "Neural architecture search: A survey," *J. Mach. Learn. Res.*, vol. 20, no. 1, pp. 1997–2017, 2019.

[30] B. Shahriari, K. Swersky, Z. Wang, R. P. Adams, and N. De Freitas, "Taking the human out of the loop: A review of bayesian optimization," *Proc. IEEE*, vol. 104, no. 1, pp. 148–175, 2015.

[31] Y. Liu, Y. Sun, B. Xue, M. Zhang, G. G. Yen, and K. C. Tan, "A survey on evolutionary neural architecture search," *IEEE Trans. Neural Netw. Learn Syst.*, vol. 34, no. 2, pp. 550–570, 2023.

[32] E. Real, S. Moore, A. Selle, S. Saxena, Y. L. Suematsu, J. Tan, Q. V. Le, and A. Kurakin, "Large-scale evolution of image classifiers," in *Proc. Int. Conf. Mach. Learn.* PMLR, 2017, pp. 2902–2911.

[33] B. Baker, O. Gupta, N. Naik, and R. Raskar, "Designing neural network architectures using reinforcement learning," in *Proc. Int. Conf. Learn. Represent.*, 2017.

[34] N. Liu, X. Ma, Z. Xu, Y. Wang, J. Tang, and J. Ye, "Autocompress: An automatic dnn structured pruning framework for ultra-high compression rates," in *Proc. AAAI Conf. Artif. Intell.*, vol. 34, no. 04, 2020, pp. 4876–4883.

[35] M. Alwani, Y. Wang, and V. Madhavan, "Decore: Deep compression with reinforcement learning," in *Proc. IEEE Conf. Comput. Vis. Pattern Recog.*, 2022, pp. 12 349–12 359.

[36] T. Zhang, S. Ye, X. Feng, X. Ma, K. Zhang, Z. Li, J. Tang, S. Liu, X. Lin, Y. Liu, M. Fardad, and Y. Wang, "Structadmm: Achieving ultrahigh efficiency in structured pruning for dnns," *IEEE Trans. Neural Netw. Learn Syst.*, vol. 33, no. 5, pp. 2259–2273, 2022.

[37] L. Liebenwein, C. Baykal, H. Lang, D. Feldman, and D. Rus, "Provable filter pruning for efficient neural networks," in *Proc. Int. Conf. Learn. Represent.*, 2020.

[38] T. Chen, B. Ji, T. Ding, B. Fang, G. Wang, Z. Zhu, L. Liang, Y. Shi, S. Yi, and X. Tu, "Only train once: A one-shot neural network training and pruning framework," in *Proc. Adv. Neural Inform. Process. Syst.*, vol. 34, 2021, pp. 19 637–19 651.

[39] G. Tian, Y. Sun, Y. Liu, X. Zeng, M. Wang, Y. Liu, J. Zhang, and J. Chen, "Adding before pruning: Sparse filter fusion for deep convolutional neural networks via auxiliary attention," *IEEE Trans. Neural Netw. Learn Syst.*, 2021.

[40] X. Ruan, Y. Liu, C. Yuan, B. Li, W. Hu, Y. Li, and S. Maybank, "Edp: An efficient decomposition and pruning scheme for convolutional neural network compression," *IEEE Trans. Neural Netw. Learn Syst.*, vol. 32, no. 10, pp. 4499–4513, 2021.

[41] Z. Wang and C. Li, "Channel pruning via lookahead search guided reinforcement learning," in *Proc. IEEE Winter Conf. Appl. Comput. Vis.*, 2022, pp. 2029–2040.

[42] Y. Sui, M. Yin, Y. Xie, H. Phan, S. Aliari Zonouz, and B. Yuan, "Chip: Channel independence-based pruning for compact neural networks," in *Proc. Adv. Neural Inform. Process. Syst.*, vol. 34, 2021, pp. 24 604–24 616.

[43] B. Dai, C. Zhu, B. Guo, and D. Wipf, "Compressing neural networks using the variational information bottleneck," in *Proc. Int. Conf. Mach. Learn.*, 2018.

[44] Z. He, Y. Qian, Y. Wang, B. Wang, X. Guan, Z. Gu, X. Ling, S. Zeng, H. Wang, and W. Zhou, "Filter pruning via feature discrimination in deep neural networks," in *Proc. Eur. Conf. Comput. Vis.* Springer, 2022, pp. 245–261.

[45] M. Lin, R. Ji, Y. Wang, Y. Zhang, B. Zhang, Y. Tian, and L. Shao, "Hrank: Filter pruning using high-rank feature map," in *Proc. IEEE Conf. Comput. Vis. Pattern Recog.*, 2020, pp. 1529–1538.

[46] Y. Zhang, M. Lin, C.-W. Lin, J. Chen, Y. Wu, Y. Tian, and R. Ji, "Carrying out cnn channel pruning in a white box," *IEEE Trans. Neural Netw. Learn Syst.*, pp. 1–10, 2022.

[47] M. Lin, R. Ji, S. Li, Y. Wang, Y. Wu, F. Huang, and Q. Ye, "Network pruning using adaptive exemplar filters," *IEEE Trans. Neural Netw. Learn Syst.*, vol. 33, no. 12, pp. 7357–7366, 2022.

[48] X. Ding, G. Ding, Y. Guo, J. Han, and C. Yan, "Approximated oracle filter pruning for destructive cnn width optimization," in *Proc. Int. Conf. Mach. Learn.*, 2019, pp. 1607–1616.

[49] M. Lin, L. Cao, Y. Zhang, L. Shao, C.-W. Lin, and R. Ji, "Pruning networks with cross-layer ranking & k-reciprocal nearest filters," *IEEE Trans. Neural Netw. Learn Syst.*, pp. 1–10, 2022.

[50] M. Lin, R. Ji, Y. Zhang, B. Zhang, Y. Wu, and Y. Tian, "Channel pruning via automatic structure search," in *Proc. Int. Joint Conf. Artif. Intell.*, 2020, pp. 673–679.

[51] W. Wang, C. Fu, J. Guo, D. Cai, and X. He, "Cop: Customized deep model compression via regularized correlation-based filter-level pruning," in *Proc. Int. Joint Conf. Artif. Intell.*, 2019, p. 3785–3791.

[52] D. Jiang, Y. Cao, and Q. Yang, "On the channel pruning using graph convolution network for convolutional neural network acceleration," in *Proc. Int. Joint Conf. Artif. Intell.*, 7 2022, pp. 3107–3113.

[53] S. Elkerdawy, M. Elhoushi, H. Zhang, and N. Ray, "Fire together wire together: A dynamic pruning approach with self-supervised mask prediction," in *Proc. IEEE Conf. Comput. Vis. Pattern Recog.*, 2022, pp. 12 454–12 463.

[54] G. Liu, K. Zhang, and M. Lv, "Soks: Automatic searching of the optimal kernel shapes for stripe-wise network pruning," *IEEE Trans. Neural Netw. Learn Syst.*, pp. 1–13, 2022.

[55] Y. Zhou, Y. Zhang, Y. Wang, and Q. Tian, "Accelerate cnn via recursive bayesian pruning," in *Proc. Int. Conf. Comput. Vis.*, 2019, pp. 3306–3315.

[56] F. Meng, H. Cheng, K. Li, H. Luo, X. Guo, G. Lu, and X. Sun, "Pruning filter in filter," in *Proc. Adv. Neural Inform. Process. Syst.*, 2020, pp. 17 629–17 640.

[57] Y. Guo, H. Yuan, J. Tan, Z. Wang, S. Yang, and J. Liu, "Gdp: Stabilized neural network pruning via gates with differentiable polarization," in *Proc. Int. Conf. Comput. Vis.*, 2021, pp. 5239–5250.

[58] M. Kang and B. Han, "Operation-aware soft channel pruning using differentiable masks," in *Proc. Int. Conf. Mach. Learn.* PMLR, 2020, pp. 5122–5131.

[59] H. Shang, J.-L. Wu, W. Hong, and C. Qian, "Neural network pruning by cooperative coevolution," in *Proc. Int. Joint Conf. Artif. Intell.*, 7 2022, pp. 4814–4820.

[60] Y. Li, S. Lin, J. Liu, Q. Ye, M. Wang, F. Chao, F. Yang, J. Ma, Q. Tian, and R. Ji, "Towards compact cnns via collaborative compression," in *Proc. IEEE Conf. Comput. Vis. Pattern Recog.*, 2021, pp. 6438–6447.

[61] Y. Zhang, S. Gao, and H. Huang, "Exploration and estimation for model compression," in *Proc. Int. Conf. Comput. Vis.*, 2021, pp. 487–496.

[62] T. Zhuang, Z. Zhang, Y. Huang, X. Zeng, K. Shuang, and X. Li, "Neuron-level structured pruning using polarization regularizer," in *Proc. Adv. Neural Inform. Process. Syst.*, vol. 33, 2020, pp. 9865–9877.

[63] S. Lin, R. Ji, C. Yan, B. Zhang, L. Cao, Q. Ye, F. Huang, and D. Doermann, "Towards optimal structured cnn pruning via generative adversarial learning," in *Proc. IEEE Conf. Comput. Vis. Pattern Recog.*, 2019, pp. 2790–2799.

[64] H. You, C. Li, P. Xu, Y. Fu, Y. Wang, X. Chen, R. G. Baraniuk, Z. Wang, and Y. Lin, "Drawing early-bird tickets: Towards more efficient training of deep networks," in *Proc. Int. Conf. Learn. Represent.*, 2020.

[65] C. Zhao, B. Ni, J. Zhang, Q. Zhao, W. Zhang, and Q. Tian, "Variational convolutional neural network pruning," in *Proc. IEEE Conf. Comput. Vis. Pattern Recog.*, 2019, pp. 2780–2789.

[66] Y. Li, S. Gu, C. Mayer, L. V. Gool, and R. Timofte, "Group sparsity: The hinge between filter pruning and decomposition for network compression," in *Proc. IEEE Conf. Comput. Vis. Pattern Recog.*, 2020, pp. 8018–8027.

[67] S. Chen and Q. Zhao, "Shallowing deep networks: Layer-wise pruning based on feature representations," *IEEE Trans. Pattern Anal. Mach. Intell.*, vol. 41, no. 12, pp. 3048–3056, 2018.

[68] X. Zhang, W. Xie, Y. Li, J. Lei, and Q. Du, "Filter pruning via learned representation median in the frequency domain," *IEEE Trans. Cybern.*, pp. 1–11, 2021.

[69] H. Li, A. Kadav, I. Durdanovic, H. Samet, and H. P. Graf, "Pruning filters for efficient convnets," in *Proc. Int. Conf. Learn. Represent.*, 2017.

[70] J. Rachwan, D. Zügner, B. Charpentier, S. Geisler, M. Ayle, and S. Günnemann, "Winning the lottery ahead of time: Efficient early network pruning," in *Proc. Int. Conf. Learn. Represent.*, 2022.

[71] L. Gonzalez-Carabarin, I. A. M. Huijben, B. Veeling, A. Schmid, and R. J. G. van Sloun, "Dynamic probabilistic pruning: A general framework for hardware-constrained pruning at different granularities," *IEEE Trans. Neural Netw. Learn Syst.*, pp. 1–12, 2022.

[72] C. Wang, R. Grosse, S. Fidler, and G. Zhang, "Eigendamage: Structured pruning in the kronecker-factored eigenbasis," in *Proc. Int. Conf. Mach. Learn.* PMLR, 2019, pp. 6566–6575.

[73] G. Ding, S. Zhang, Z. Jia, J. Zhong, and J. Han, "Where to prune: Using lstm to guide data-dependent soft pruning," *IEEE Trans. Image Process.*, vol. 30, pp. 293–304, 2021.

[74] Z. Zhuang, M. Tan, B. Zhuang, J. Liu, Y. Guo, Q. Wu, J. Huang, and J. Zhu, "Discrimination-aware channel pruning for deep neural networks," in *Proc. Adv. Neural Inform. Process. Syst.*, 2018, p. 883–894.

[75] M. Nonnenmacher, T. Pfeil, I. Steinwart, and D. Reeb, "Sosp: Efficiently capturing global correlations by second-order structured pruning," in *Proc. Int. Conf. Learn. Represent.*, 2022.

[76] Z. Chen, T.-B. Xu, C. Du, C.-L. Liu, and H. He, "Dynamical channel pruning by conditional accuracy change for deep neural networks," *IEEE Trans. Neural Netw. Learn Syst.*, vol. 32, no. 2, pp. 799–813, 2021.

[77] Z. Liu, J. Li, Z. Shen, G. Huang, S. Yan, and C. Zhang, "Learning efficient convolutional networks through network slimming," in *Proc. Int. Conf. Comput. Vis.*, 2017, pp. 2736–2744.

[78] M. Alizadeh, S. A. Tailor, L. M. Zintgraf, J. van Amersfoort, S. Farquhar, N. D. Lane, and Y. Gal, "Prospect pruning: Finding trainable weights at initialization using meta-gradients," in *Proc. Int. Conf. Learn. Represent.*, 2022.

[79] X. Ning, T. Zhao, W. Li, P. Lei, Y. Wang, and H. Yang, "Dsa: More efficient budgeted pruning via differentiable sparsity allocation," in *Proc. Eur. Conf. Comput. Vis.* Springer, 2020, pp. 592–607.

[80] Y. Tang, Y. Wang, Y. Xu, D. Tao, C. XU, C. Xu, and C. Xu, "Scop: Scientific control for reliable neural network pruning," in *Proc. Adv. Neural Inform. Process. Syst.*, 2020, pp. 10 936–10 947.

[81] Y. Tang, Y. Wang, Y. Xu, Y. Deng, C. Xu, D. Tao, and C. Xu, "Manifold regularized dynamic network pruning," in *Proc. IEEE Conf. Comput. Vis. Pattern Recog.*, 2021, pp. 5018–5028.

[82] Y. He, P. Liu, Z. Wang, Z. Hu, and Y. Yang, "Filter pruning via geometric median for deep convolutional neural networks acceleration," in *Proc. IEEE Conf. Comput. Vis. Pattern Recog.*, 2019, pp. 4340–4349.

[83] F. Li, G. Li, X. He, and J. Cheng, "Dynamic dual gating neural networks," in *Proc. Int. Conf. Comput. Vis.*, 2021, pp. 5330–5339.

[84] Y. Guan, N. Liu, P. Zhao, Z. Che, K. Bian, Y. Wang, and J. Tang, "Dais: Automatic channel pruning via differentiable annealing indicator search," *IEEE Trans. Neural Netw. Learn Syst.*, pp. 1–12, 2022.

[85] S. Yu, A. Mazaheri, and A. Jannesari, "Topology-aware network pruning using multi-stage graph embedding and reinforcement learning," in *Proc. Int. Conf. Mach. Learn.* PMLR, 2022, pp. 25 656–25 667.

[86] ——, "Auto graph encoder-decoder for neural network pruning," in *Proc. Int. Conf. Comput. Vis.*, 2021, pp. 6362–6372.

[87] Z. Wang, C. Li, and X. Wang, "Convolutional neural network pruning with structural redundancy reduction," in *Proc. IEEE Conf. Comput. Vis. Pattern Recog.*, 2021, pp. 14 913–14 922.

[88] X. Dong and Y. Yang, "Network pruning via transformable architecture search," in *Proc. Adv. Neural Inform. Process. Syst.*, 2019, pp. 760–771.

[89] S. Zhong, G. Zhang, N. Huang, and S. Xu, "Revisit kernel pruning with lottery regulated grouped convolutions," in *Proc. Int. Conf. Learn. Represent.*, 2022.

[90] Y. He, G. Kang, X. Dong, Y. Fu, and Y. Yang, "Soft filter pruning for accelerating deep convolutional neural networks," in *Proc. Int. Joint Conf. Artif. Intell.*, 2018, p. 2234–2240.

[91] Y. He, P. Liu, L. Zhu, and Y. Yang, "Filter pruning by switching to neighboring cnns with good attributes," *IEEE Trans. Neural Netw. Learn Syst.*, pp. 1–13, 2022.

[92] Y. He, Y. Ding, P. Liu, L. Zhu, H. Zhang, and Y. Yang, "Learning filter pruning criteria for deep convolutional neural networks

acceleration," in *Proc. IEEE Conf. Comput. Vis. Pattern Recog.*, 2020, pp. 2009–2018.
[93] X. Ding, T. Hao, J. Tan, J. Liu, J. Han, Y. Guo, and G. Ding, "Resrep: Lossless cnn pruning via decoupling remembering and forgetting," in *Proc. Int. Conf. Comput. Vis.*, 2021, pp. 4510–4520.
[94] Z. You, K. Yan, J. Ye, M. Ma, and P. Wang, "Gate decorator: Global filter pruning method for accelerating deep convolutional neural networks," in *Proc. Adv. Neural Inform. Process. Syst.*, 2019.
[95] S. Lee and B. C. Song, "Ensemble knowledge guided sub-network search and fine-tuning for filter pruning," in *Proc. Eur. Conf. Comput. Vis.* Springer, 2022, pp. 569–585.
[96] X. Ding, G. Ding, Y. Guo, and J. Han, "Centripetal sgd for pruning very deep convolutional networks with complicated structure," in *Proc. IEEE Conf. Comput. Vis. Pattern Recog.*, 2019.
[97] H. Wang, C. Qin, Y. Zhang, and Y. Fu, "Neural pruning via growing regularization," in *Proc. Int. Conf. Learn. Represent.*, 2022.
[98] T.-W. Chin, R. Ding, C. Zhang, and D. Marculescu, "Towards efficient model compression via learned global ranking," in *Proc. IEEE Conf. Comput. Vis. Pattern Recog.*, 2020, pp. 1518–1528.
[99] H. Peng, J. Wu, S. Chen, and J. Huang, "Collaborative channel pruning for deep networks," in *Proc. Int. Conf. Mach. Learn.* PMLR, 2019, pp. 5113–5122.
[100] S. Gao, F. Huang, Y. Zhang, and H. Huang, "Disentangled differentiable network pruning," in *Proc. Eur. Conf. Comput. Vis.* Springer, 2022, pp. 328–345.
[101] B. Li, B. Wu, J. Su, and G. Wang, "Eagleeye: Fast sub-net evaluation for efficient neural network pruning," in *Proc. Eur. Conf. Comput. Vis.* Springer, 2020, pp. 639–654.
[102] S. Gao, F. Huang, J. Pei, and H. Huang, "Discrete model compression with resource constraint for deep neural networks," in *Proc. IEEE Conf. Comput. Vis. Pattern Recog.*, 2020, pp. 1899–1908.
[103] Y. He, J. Lin, Z. Liu, H. Wang, L.-J. Li, and S. Han, "Amc: Automl for model compression and acceleration on mobile devices," in *Proc. Eur. Conf. Comput. Vis.*, 2018, pp. 784–800.
[104] H. Fan, J. Mu, and W. Zhang, "Bayesian optimization with clustering and rollback for cnn auto pruning," in *Proc. Eur. Conf. Comput. Vis.* Springer, 2022, pp. 494–511.
[105] Y. Li, K. Adamczewski, W. Li, S. Gu, R. Timofte, and L. Van Gool, "Revisiting random channel pruning for neural network compression," in *Proc. IEEE Conf. Comput. Vis. Pattern Recog.*, 2022, pp. 191–201.
[106] R. Yu, A. Li, C.-F. Chen, J.-H. Lai, V. I. Morariu, X. Han, M. Gao, C.-Y. Lin, and L. S. Davis, "Nisp: Pruning networks using neuron importance score propagation," in *Proc. IEEE Conf. Comput. Vis. Pattern Recog.*, 2018, pp. 9194–9203.
[107] S. Yu, Z. Yao, A. Gholami, Z. Dong, S. Kim, M. W. Mahoney, and K. Keutzer, "Hessian-aware pruning and optimal neural implant," in *Proc. IEEE Winter Conf. Appl. Comput. Vis.*, 2022, pp. 3880–3891.
[108] J. Li, Q. Qi, J. Wang, C. Ge, Y. Li, Z. Yue, and H. Sun, "Oicsr: Out-in-channel sparsity regularization for compact deep neural networks," in *Proc. IEEE Conf. Comput. Vis. Pattern Recog.*, 2019, pp. 7046–7055.
[109] Y.-J. Zheng, S.-B. Chen, C. H. Q. Ding, and B. Luo, "Model compression based on differentiable network channel pruning," *IEEE Trans. Neural Netw. Learn Syst.*, pp. 1–10, 2022.
[110] J. Meng, L. Yang, J. Shin, D. Fan, and J.-s. Seo, "Contrastive dual gating: Learning sparse features with contrastive learning," in *Proc. IEEE Conf. Comput. Vis. Pattern Recog.*, 2022, pp. 12 257–12 265.
[111] H. Salehinejad and S. Valaee, "Edropout: Energy-based dropout and pruning of deep neural networks," *IEEE Trans. Neural Netw. Learn Syst.*, vol. 33, no. 10, pp. 5279–5292, 2022.
[112] C. Peng, Y. Li, R. Shang, and L. Jiao, "Recnas: Resource-constrained neural architecture search based on differentiable annealing and dynamic pruning," *IEEE Trans. Neural Netw. Learn Syst.*, pp. 1–15, 2022.
[113] S. Lin, R. Ji, Y. Li, Y. Wu, F. Huang, and B. Zhang, "Accelerating convolutional networks via global & dynamic filter pruning," in *Proc. Int. Joint Conf. Artif. Intell.*, vol. 2, no. 7. Stockholm, 2018, p. 8.
[114] P. Molchanov, A. Mallya, S. Tyree, I. Frosio, and J. Kautz, "Importance estimation for neural network pruning," in *Proc. IEEE Conf. Comput. Vis. Pattern Recog.*, 2019, pp. 11 264–11 272.
[115] J.-H. Luo, J. Wu, and W. Lin, "Thinet: A filter level pruning method for deep neural network compression," in *Proc. IEEE Conf. Comput. Vis. Pattern Recog.*, 2017, pp. 5058–5066.
[116] L. Liu, L. Deng, X. Hu, M. Zhu, G. Li, Y. Ding, and Y. Xie, "Dynamic sparse graph for efficient deep learning," in *Proc. Int. Conf. Learn. Represent.*, 2019.
[117] Z. Huang and N. Wang, "Data-driven sparse structure selection for deep neural networks," in *Proc. Eur. Conf. Comput. Vis.*, 2018, pp. 304–320.
[118] W. Kim, S. Kim, M. Park, and G. Jeon, "Neuron merging: Compensating for pruned neurons," in *Proc. Adv. Neural Inform. Process. Syst.*, 2020, pp. 585–595.
[119] X. Gao, Y. Zhao, Ł. Dudziak, R. Mullins, and C.-z. Xu, "Dynamic channel pruning: Feature boosting and suppression," in *Proc. Int. Conf. Learn. Represent.*, 2019.
[120] J. Chen, S. Chen, and S. J. Pan, "Storage efficient and dynamic flexible runtime channel pruning via deep reinforcement learning," in *Proc. Adv. Neural Inform. Process. Syst.*, vol. 33, 2020, pp. 14 747–14 758.
[121] S. Guo, Y. Wang, Q. Li, and J. Yan, "Dmcp: Differentiable markov channel pruning for neural networks," in *Proc. IEEE Conf. Comput. Vis. Pattern Recog.*, 2020, pp. 1539–1547.
[122] Y. Wang, Y. Lu, and T. Blankevoort, "Differentiable joint pruning and quantization for hardware efficiency," in *Proc. Eur. Conf. Comput. Vis.*, 2020, pp. 259–277.
[123] Z. Hou, M. Qin, F. Sun, X. Ma, K. Yuan, Y. Xu, Y.-K. Chen, R. Jin, Y. Xie, and S.-Y. Kung, "Chex: Channel exploration for cnn model compression," in *Proc. IEEE Conf. Comput. Vis. Pattern Recog.*, 2022, pp. 12 287–12 298.
[124] M. Ye, C. Gong, L. Nie, D. Zhou, A. Klivans, and Q. Liu, "Good subnetworks provably exist: Pruning via greedy forward selection," in *Proc. Int. Conf. Mach. Learn.* PMLR, 2020, pp. 10 820–10 830.
[125] M. Shen, P. Molchanov, H. Yin, and J. M. Alvarez, "When to prune? a policy towards early structural pruning," in *Proc. IEEE Conf. Comput. Vis. Pattern Recog.*, 2022, pp. 12 247–12 256.
[126] Z. Liu, X. Zhang, Z. Shen, Y. Wei, K.-T. Cheng, and J. Sun, "Joint multi-dimension pruning via numerical gradient update," *IEEE Trans. Image Process.*, vol. 30, pp. 8034–8045, 2021.
[127] R. Humble, M. Shen, J. A. Latorre, E. Darve, and J. Alvarez, "Soft masking for cost-constrained channel pruning," in *Proc. Eur. Conf. Comput. Vis.* Springer, 2022, pp. 641–657.
[128] Z. Liu, H. Mu, X. Zhang, Z. Guo, X. Yang, K.-T. Cheng, and J. Sun, "Metapruning: Meta learning for automatic neural network channel pruning," in *Proc. Int. Conf. Comput. Vis.*, 2019, pp. 3296–3305.
[129] Y. Li, P. Zhao, G. Yuan, X. Lin, Y. Wang, and X. Chen, "Pruning-as-search: Efficient neural architecture search via channel pruning and structural reparameterization," in *Proc. Int. Joint Conf. Artif. Intell.*, 7 2022, pp. 3236–3242.
[130] L. Liu, S. Zhang, Z. Kuang, A. Zhou, J.-H. Xue, X. Wang, Y. Chen, W. Yang, Q. Liao, and W. Zhang, "Group fisher pruning for practical network compression," in *Proc. Int. Conf. Mach. Learn.* PMLR, 2021, pp. 7021–7032.
[131] M. Lin, Y. Zhang, Y. Li, B. Chen, F. Chao, M. Wang, S. Li, Y. Tian, and R. Ji, "1xn pattern for pruning convolutional neural networks," *IEEE Trans. Pattern Anal. Mach. Intell.*, 2022.
[132] J. Ye, X. Lu, Z. Lin, and J. Z. Wang, "Rethinking the smaller-norm-less-informative assumption in channel pruning of convolution layers," in *Proc. Int. Conf. Learn. Represent.*, 2018.
[133] Z. Li, G. Yuan, W. Niu, P. Zhao, Y. Li, Y. Cai, X. Shen, Z. Zhan, Z. Kong, Q. Jin, Z. Chen, S. Liu, K. Yang, B. Ren, Y. Wang, and X. Lin, "Npas: A compiler-aware framework of unified network pruning and architecture search for beyond real-time mobile acceleration," in *Proc. IEEE Conf. Comput. Vis. Pattern Recog.*, 2021, pp. 14 255–14 266.
[134] H. You, B. Li, Z. Sun, X. Ouyang, and Y. Lin, "Supertickets: Drawing task-agnostic lottery tickets from supernets via jointly architecture searching and parameter pruning," in *Proc. Eur. Conf. Comput. Vis.* Springer, 2022, pp. 674–690.
